# Supplementary material for: Feature Selection Methods for Cost-Constrained Classification in Random Forests
Source: arXiv:2008.06298 ancillary file (2020-08-17)
Supplement: Supplementary file 1 [file Additional_file_2.pdf]

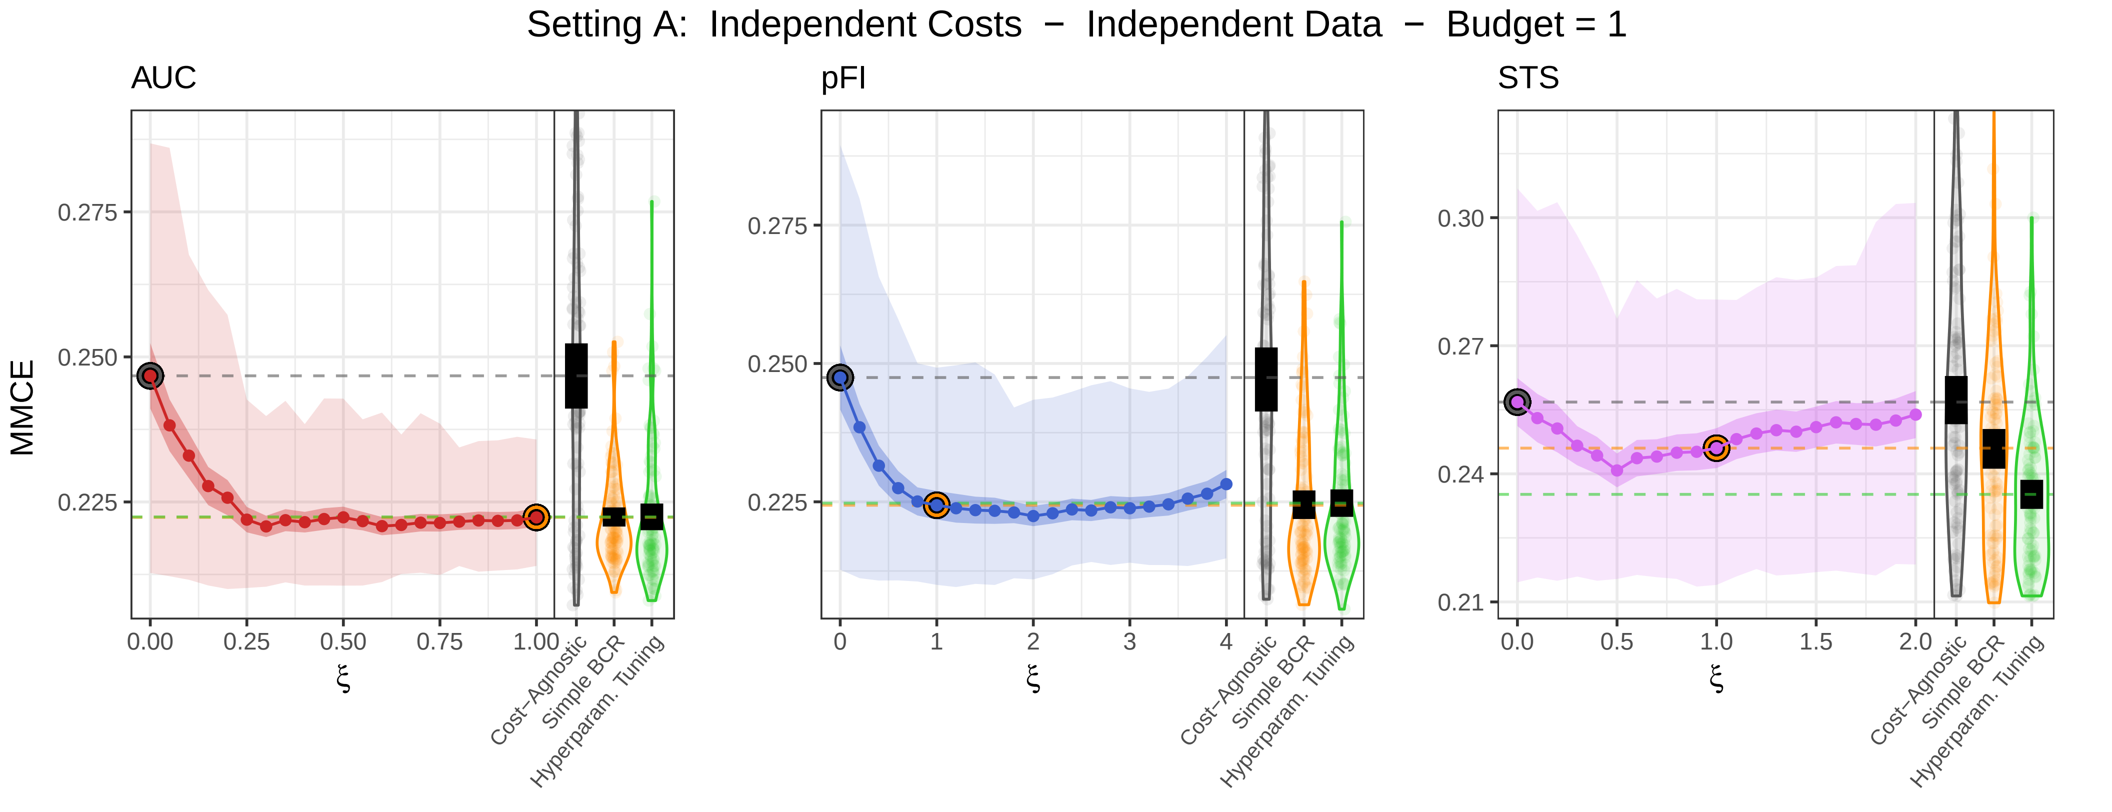

Setting A: Independent Costs − Independent Data − Budget = 1
AUC
pFI
STS
MMCE
0.275
0.250
0.225
0.30
0.27
0.24
0.21
0.00
0.25
0.50
0.75
1.00
0
1
2
3
4
0.0
0.5
1.0
1.5
2.0
ξ
Cost−Agnostic
Simple BCR
Hyperparam. Tuning

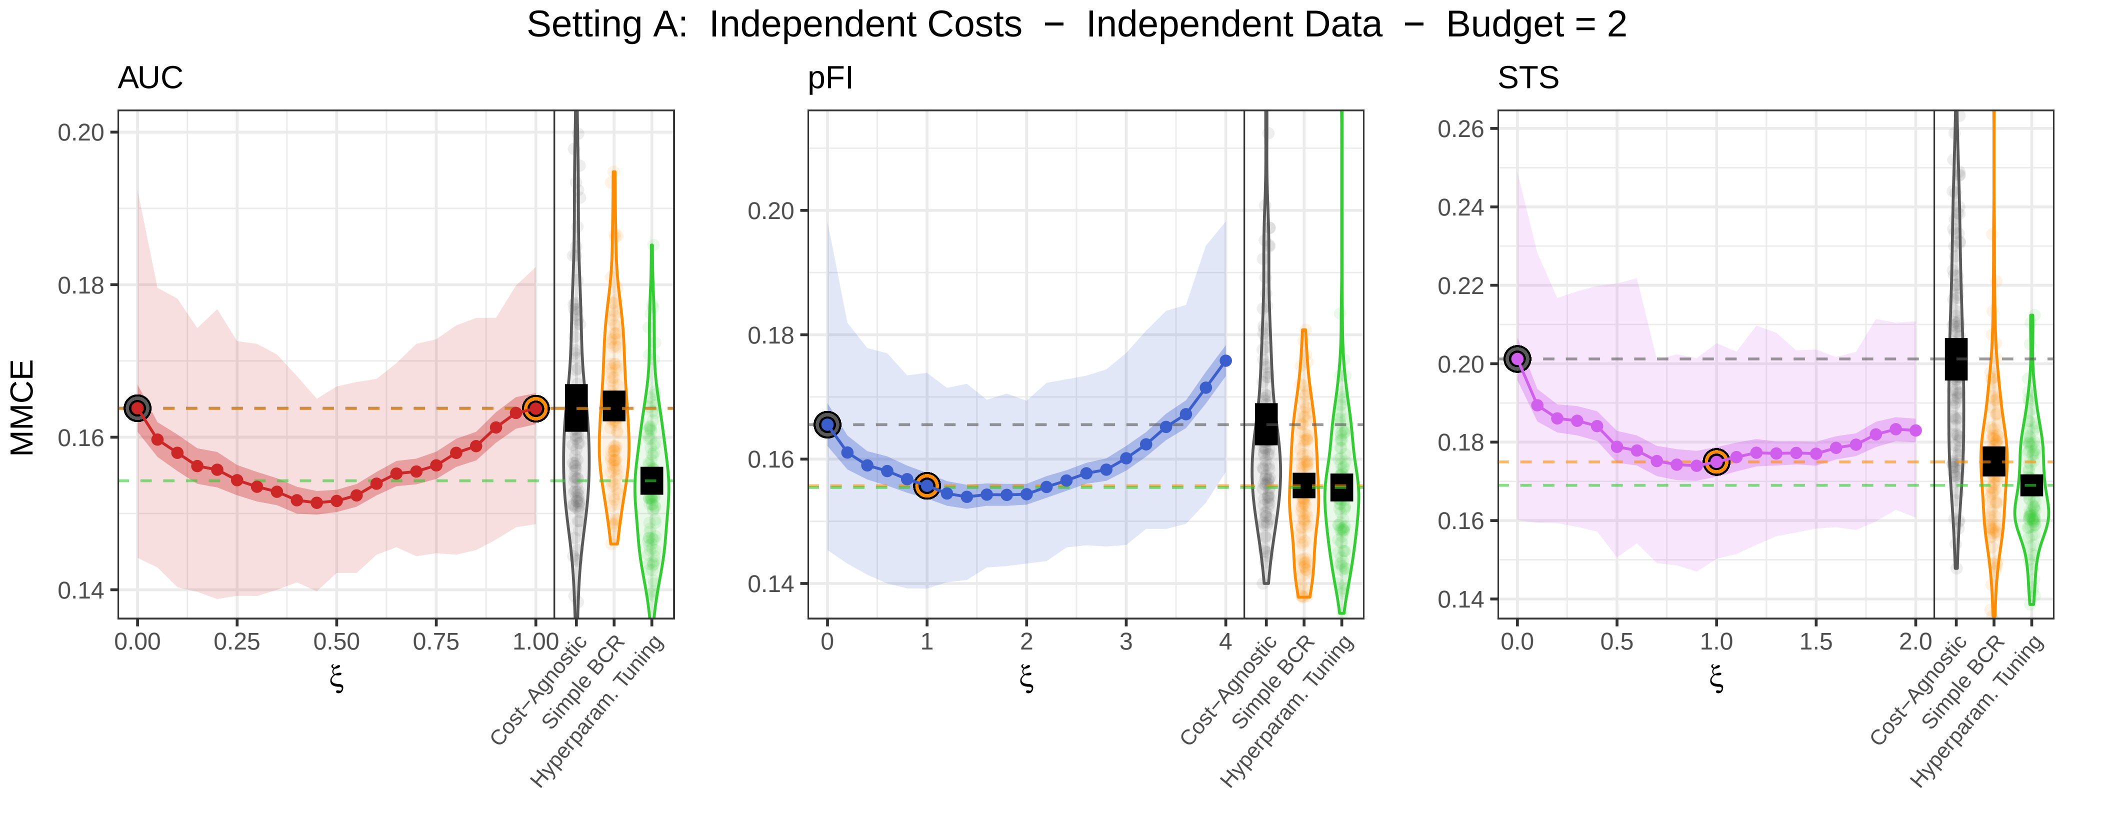

Setting A: Independent Costs − Independent Data − Budget = 2
AUC
pFI
STS
MMCE
ξ
Cost−Agnostic
Simple BCR
Hyperparam. Tuning
0.20
0.18
0.16
0.14
0.00
0.25
0.50
0.75
1.00
0
1
2
3
4
0.26
0.24
0.22
0.0
0.5
1.0
1.5
2.0

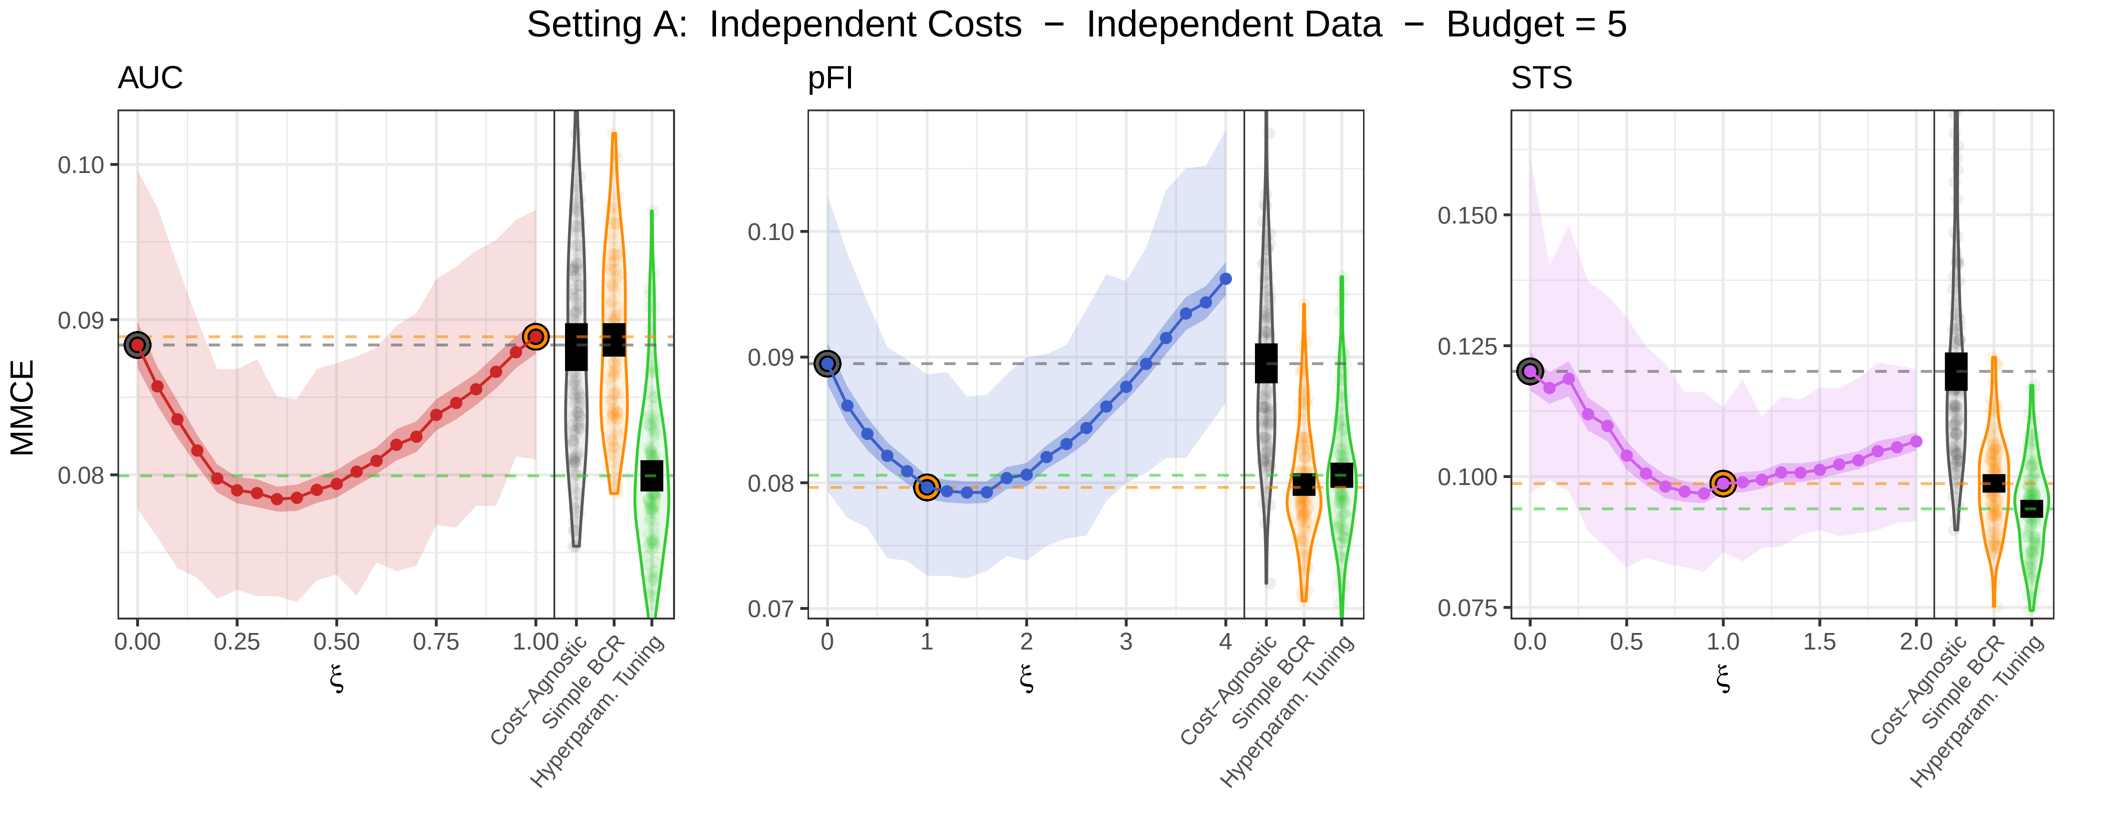
Setting A: Independent Costs − Independent Data − Budget = 5
AUC
pFI
STS
MMCE
0.10
0.09
0.08
0.00
0.25
0.50
0.75
1.00
0.10
0.09
0.08
0.07
0
1
2
3
4
0.150
0.125
0.100
0.075
0.0
0.5
1.0
1.5
2.0
ξ
Cost−Agnostic
Simple BCR
Hyperparam. Tuning

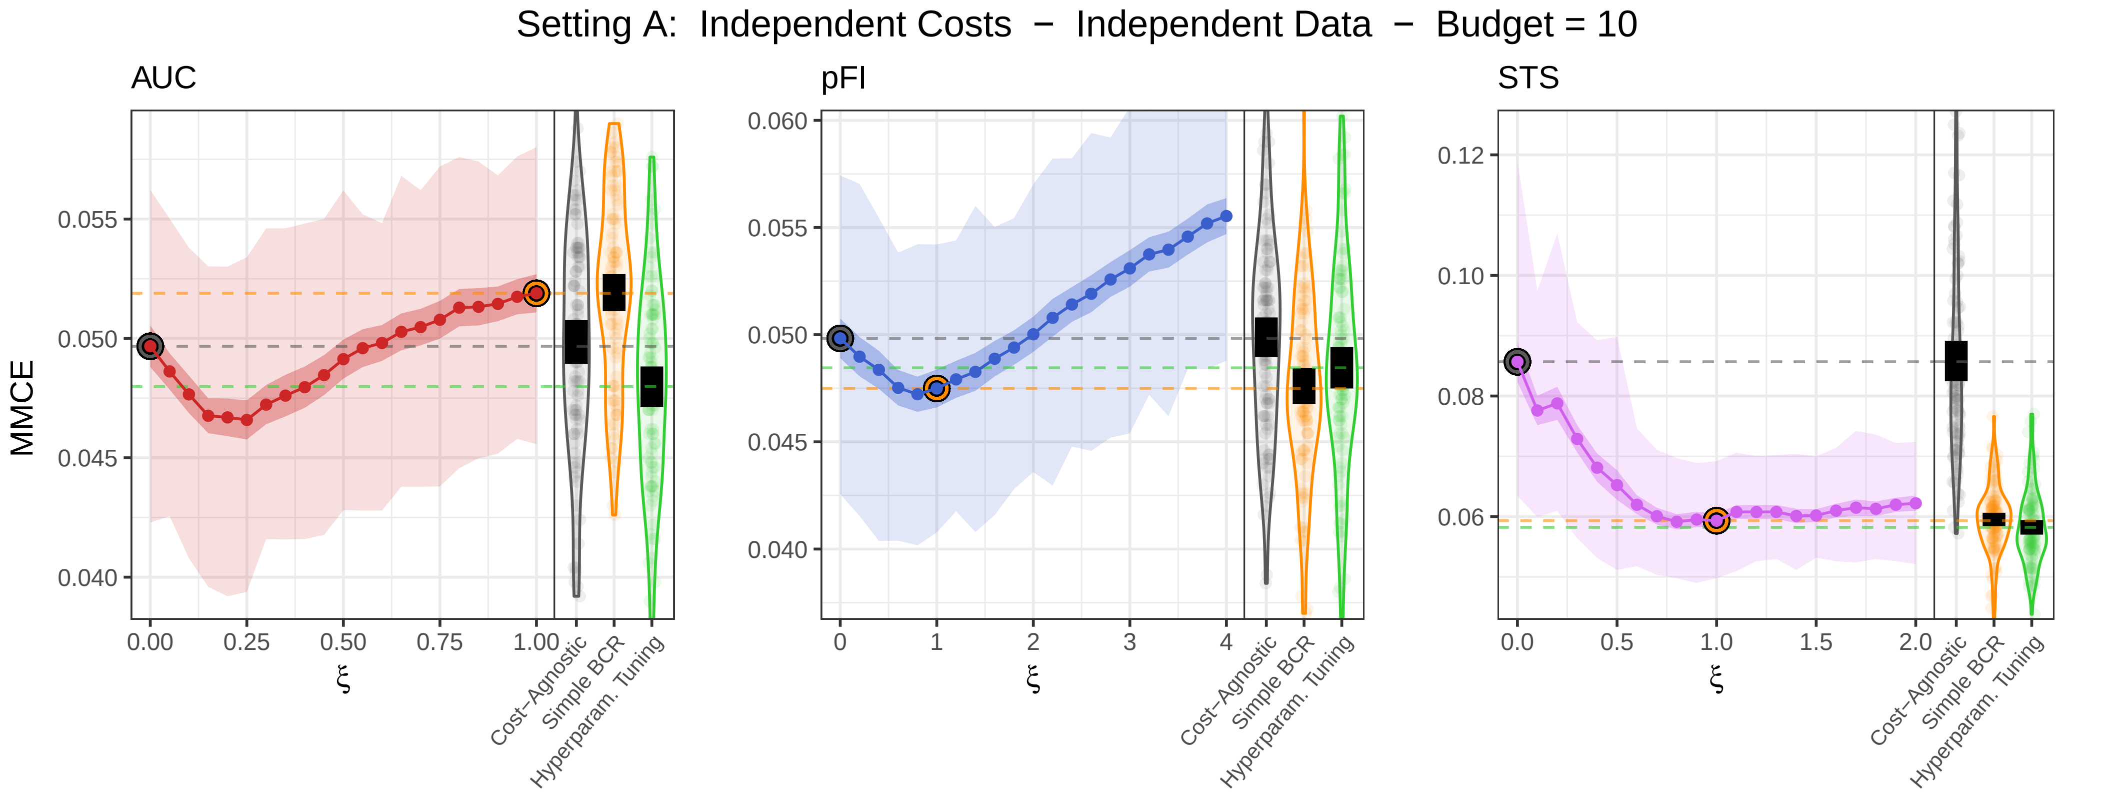
Setting A: Independent Costs − Independent Data − Budget = 10
AUC
pFI
STS
MMCE
0.055
0.050
0.045
0.040
0.060
0.12
0.10
0.08
0.06
0.00
0.25
0.50
0.75
1.00
0
1
2
3
4
0.0
0.5
1.0
1.5
2.0
ξ
Cost−Agnostic
Simple BCR
Hyperparam. Tuning

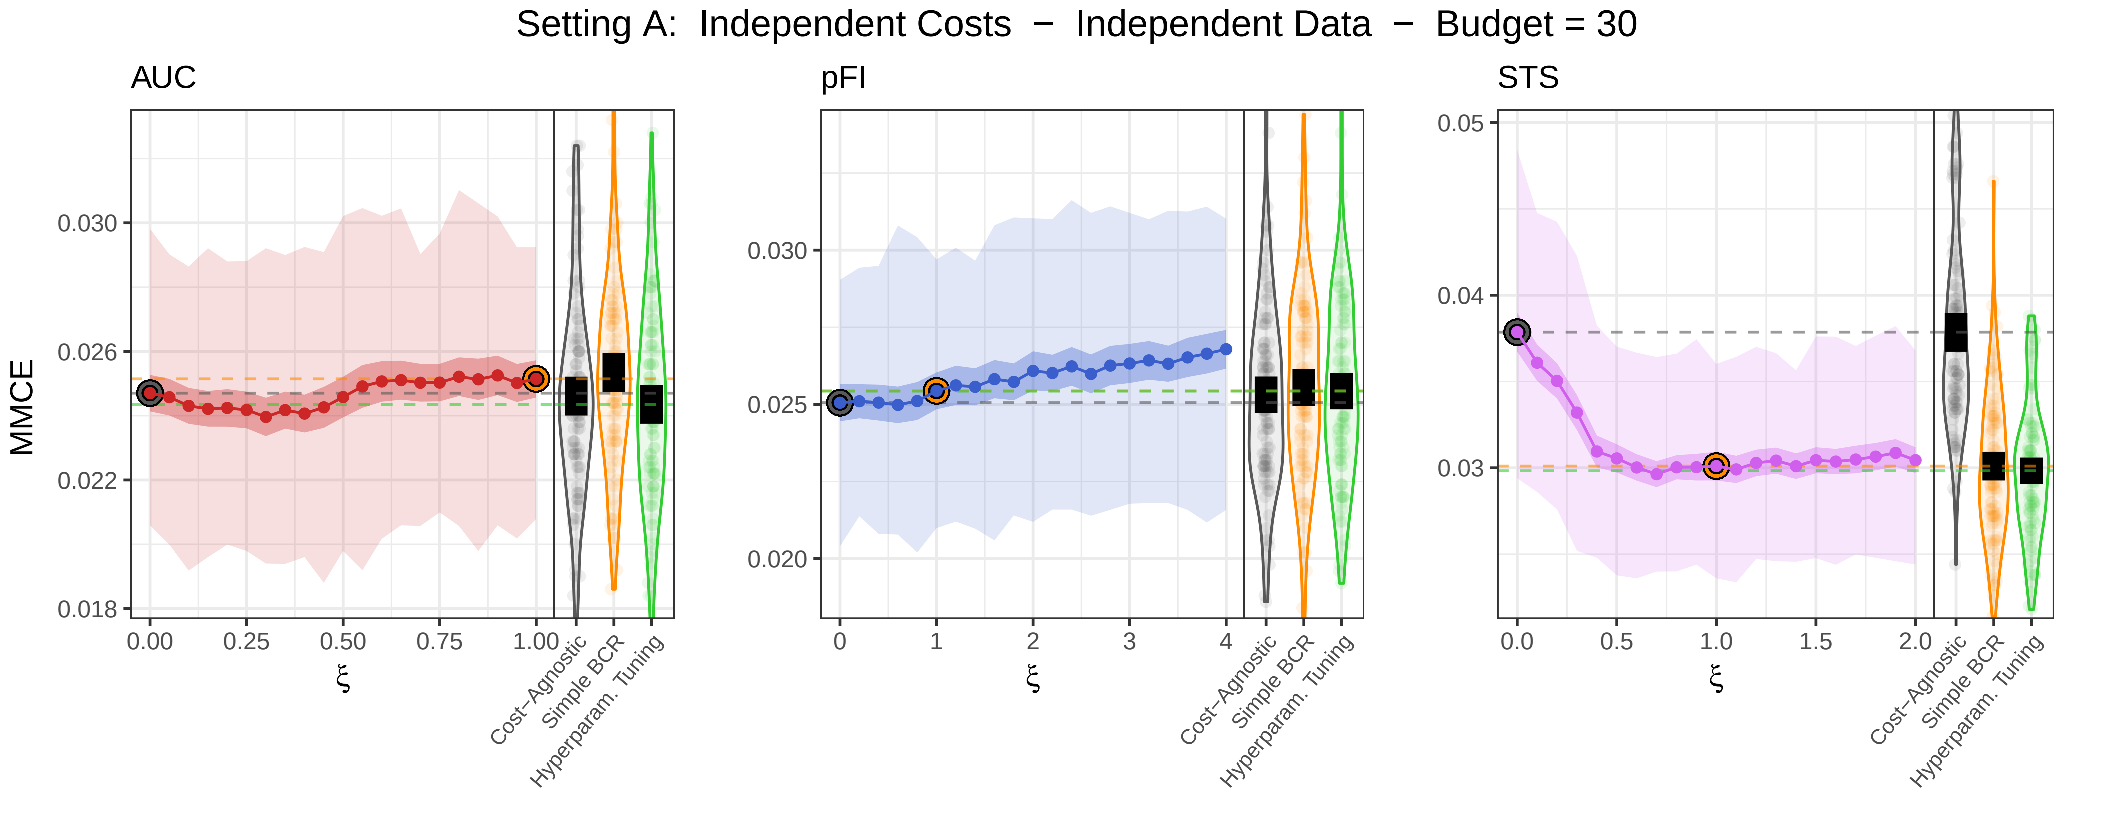
Setting A: Independent Costs − Independent Data − Budget = 30
AUC
pFI
STS
MMCE
0.030
0.026
0.022
0.018
0.00
0.25
0.50
0.75
1.00
0.020
0.025
0.030
0
1
2
3
4
0.03
0.04
0.05
0.0
0.5
1.0
1.5
2.0
ξ
Cost−Agnostic
Simple BCR
Hyperparam. Tuning

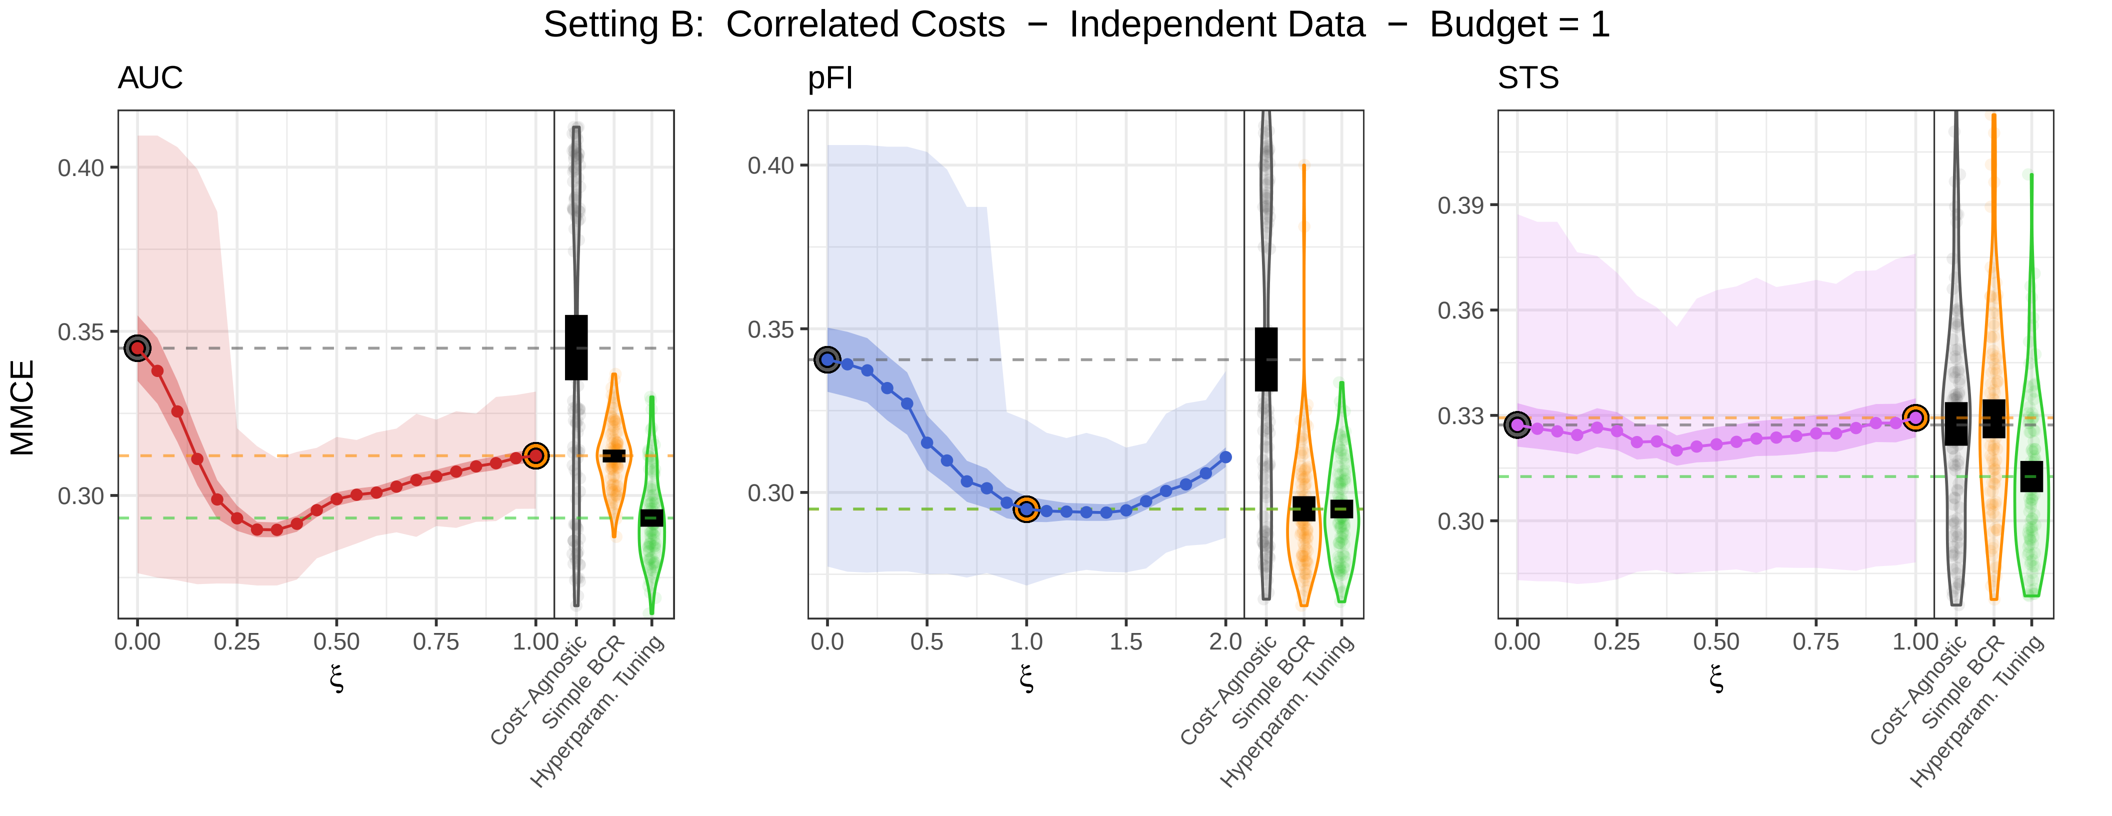
Setting B: Correlated Costs − Independent Data − Budget = 1
AUC
pFI
STS
MMCE
ξ
Cost−Agnostic
Simple BCR
Hyperparam. Tuning
0.00
0.25
0.50
0.75
1.00
0.0
0.5
1.0
1.5
2.0
0.30
0.35
0.40
0.33
0.36
0.39

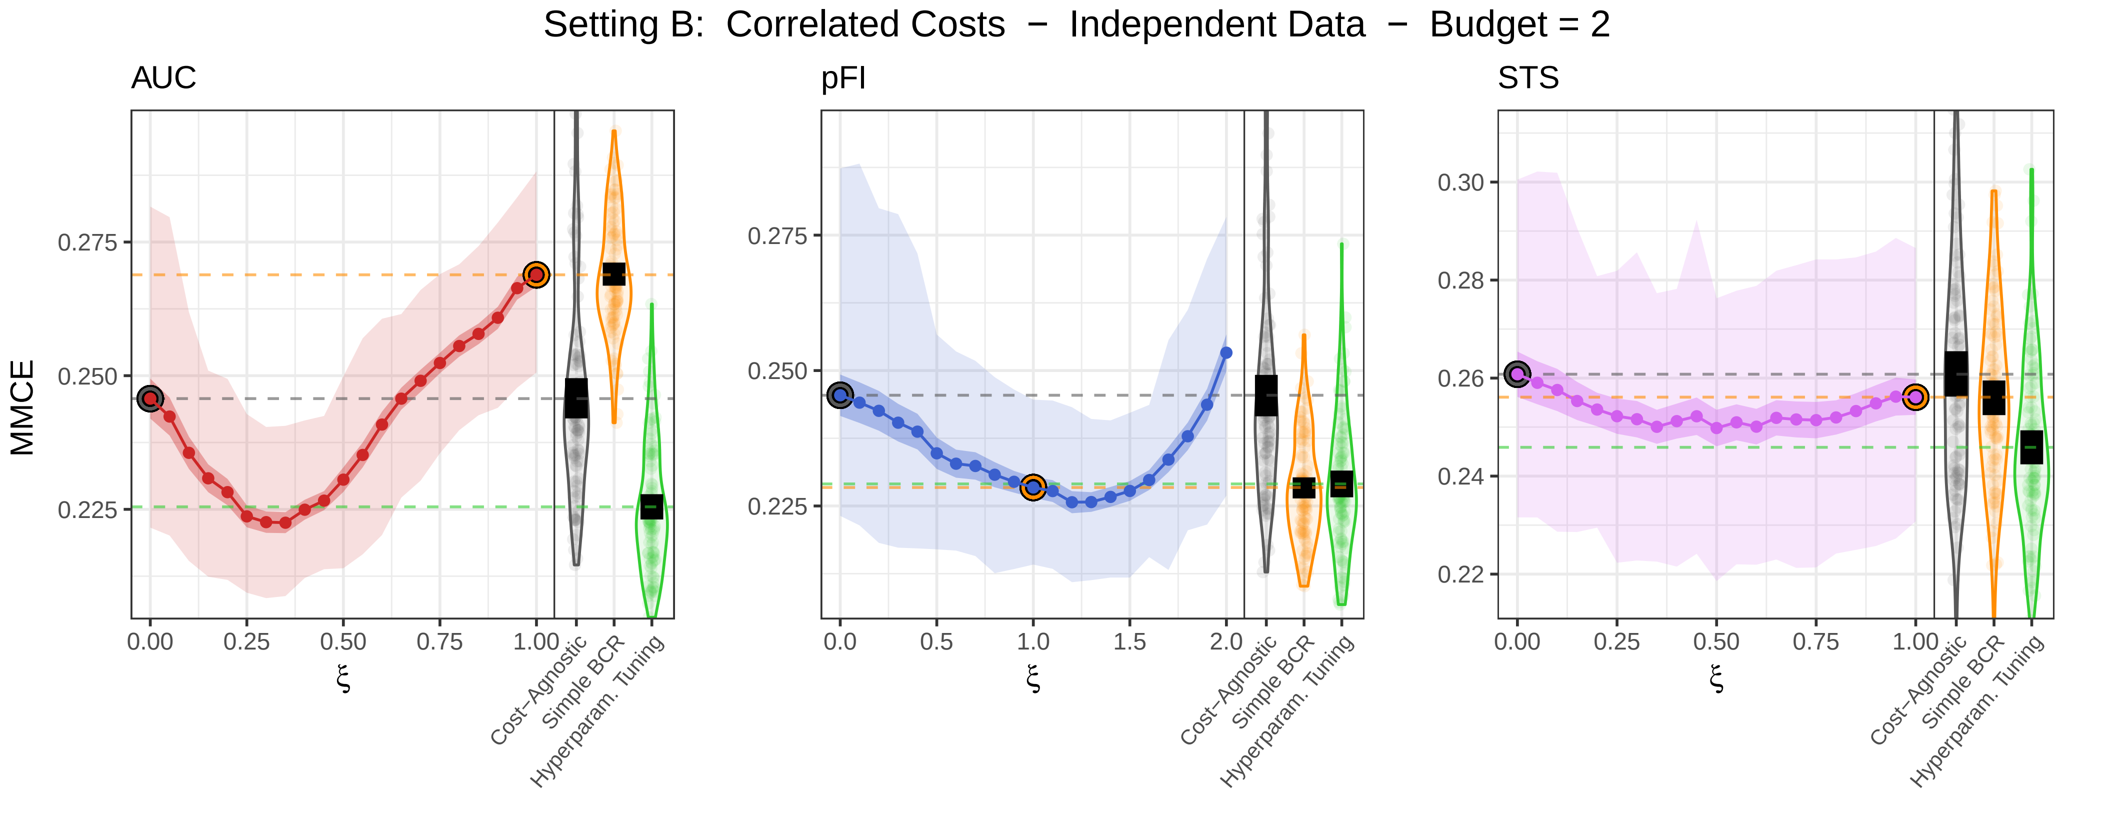

Setting B: Correlated Costs − Independent Data − Budget = 2
AUC
pFI
STS
MMCE
0.275
0.250
0.225
0.30
0.28
0.26
0.24
0.22
0.00
0.25
0.50
0.75
1.00
0.0
0.5
1.0
1.5
2.0
ξ
Cost−Agnostic
Simple BCR
Hyperparam. Tuning

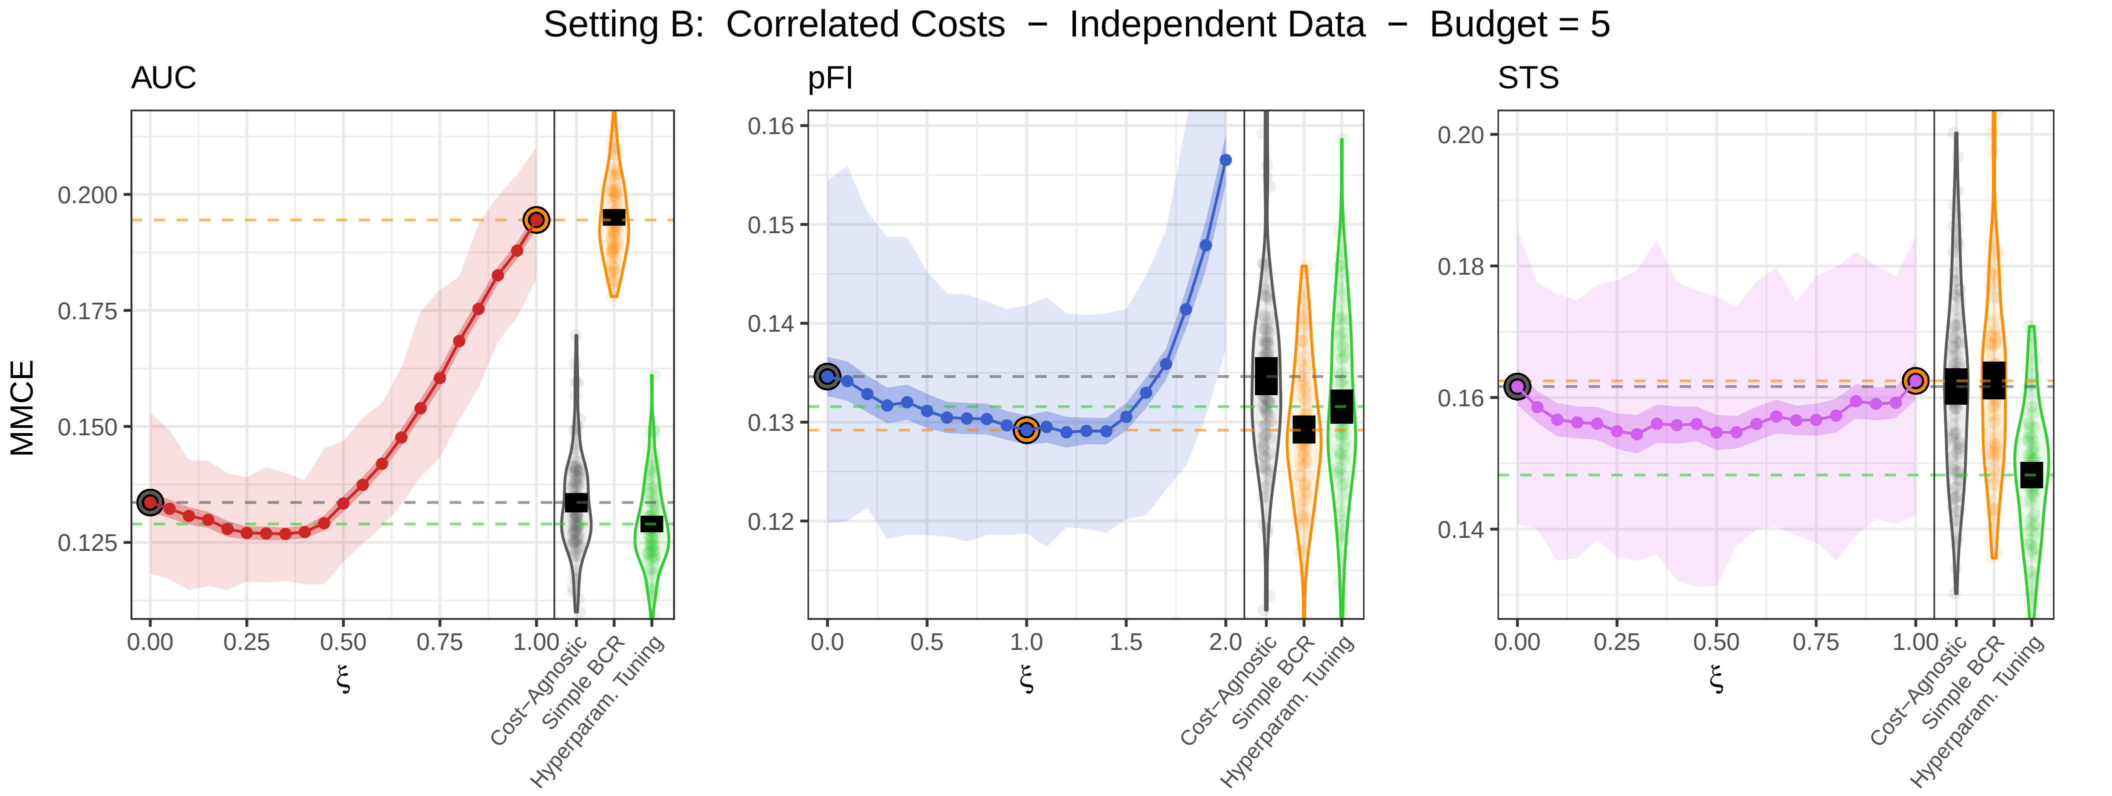

Setting B: Correlated Costs − Independent Data − Budget = 5
AUC
pFI
STS
MMCE
0.200
0.175
0.150
0.125
0.16
0.15
0.14
0.13
0.12
0.20
0.18
0.16
0.14
0.00
0.25
0.50
0.75
1.00
0.0
0.5
1.0
1.5
2.0
ξ
Cost−Agnostic
Simple BCR
Hyperparam. Tuning

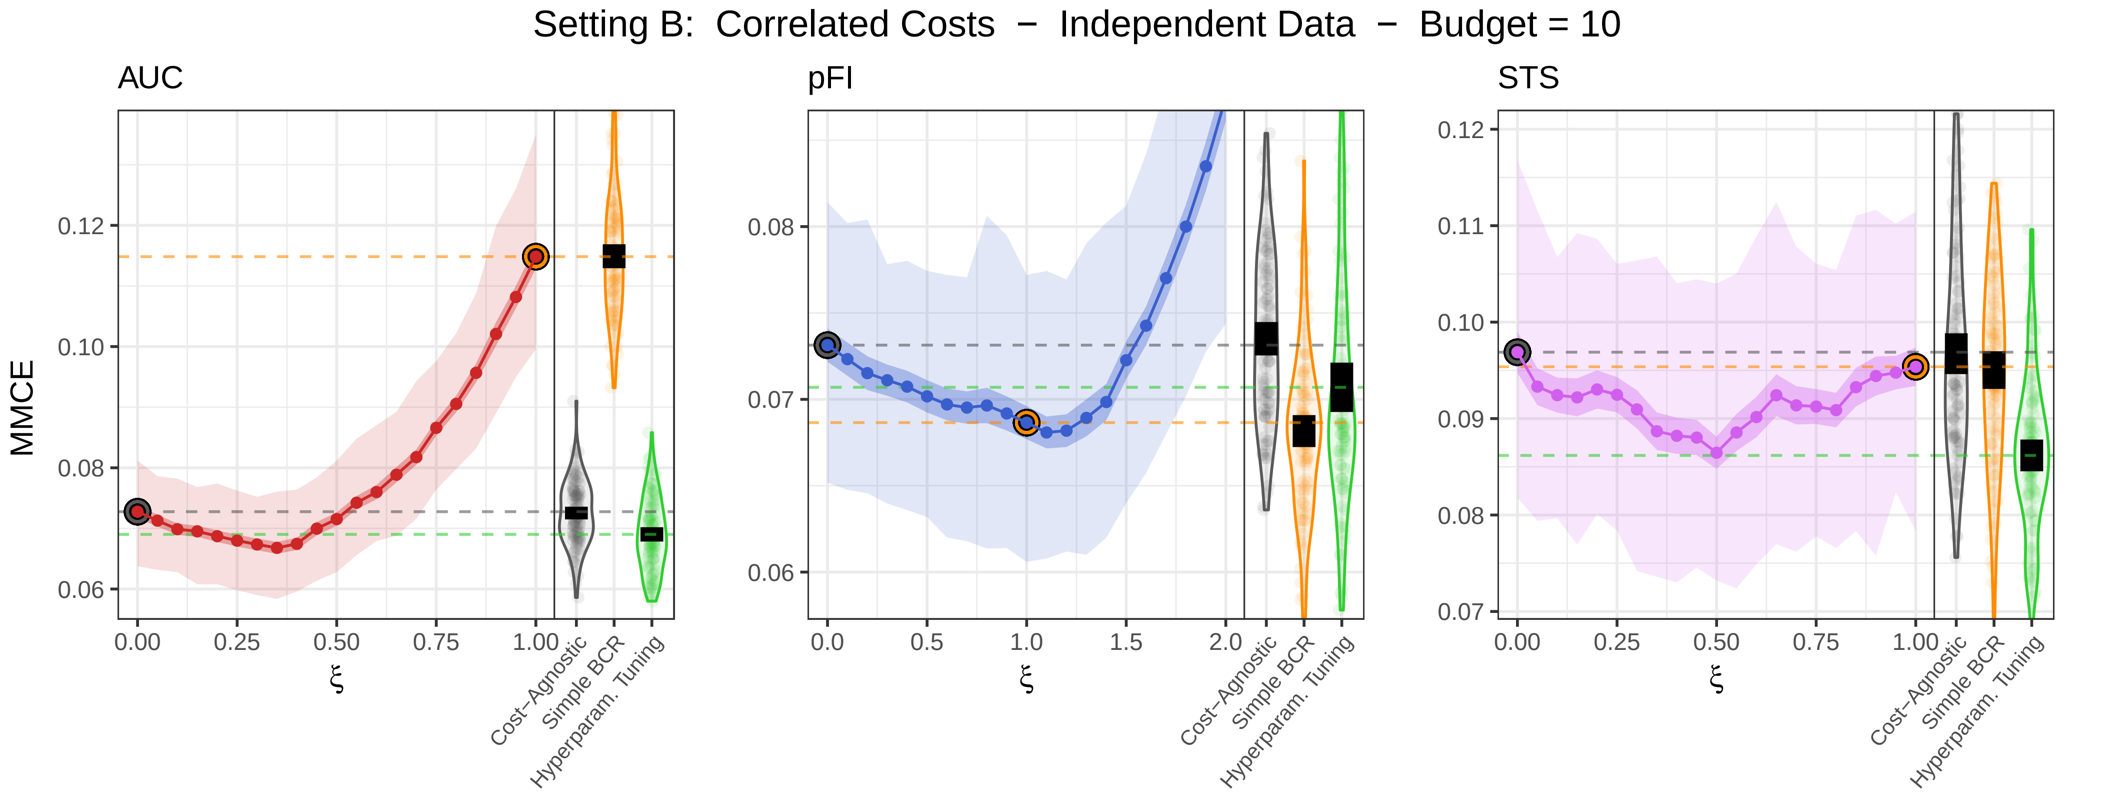

Setting B: Correlated Costs − Independent Data − Budget = 10
AUC
pFI
STS
MMCE
ξ
0.00
0.25
0.50
0.75
1.00
0.0
0.5
1.0
1.5
2.0
0.06
0.08
0.10
0.12
0.07
0.09
0.11
Cost−Agnostic
Simple BCR
Hyperparam. Tuning

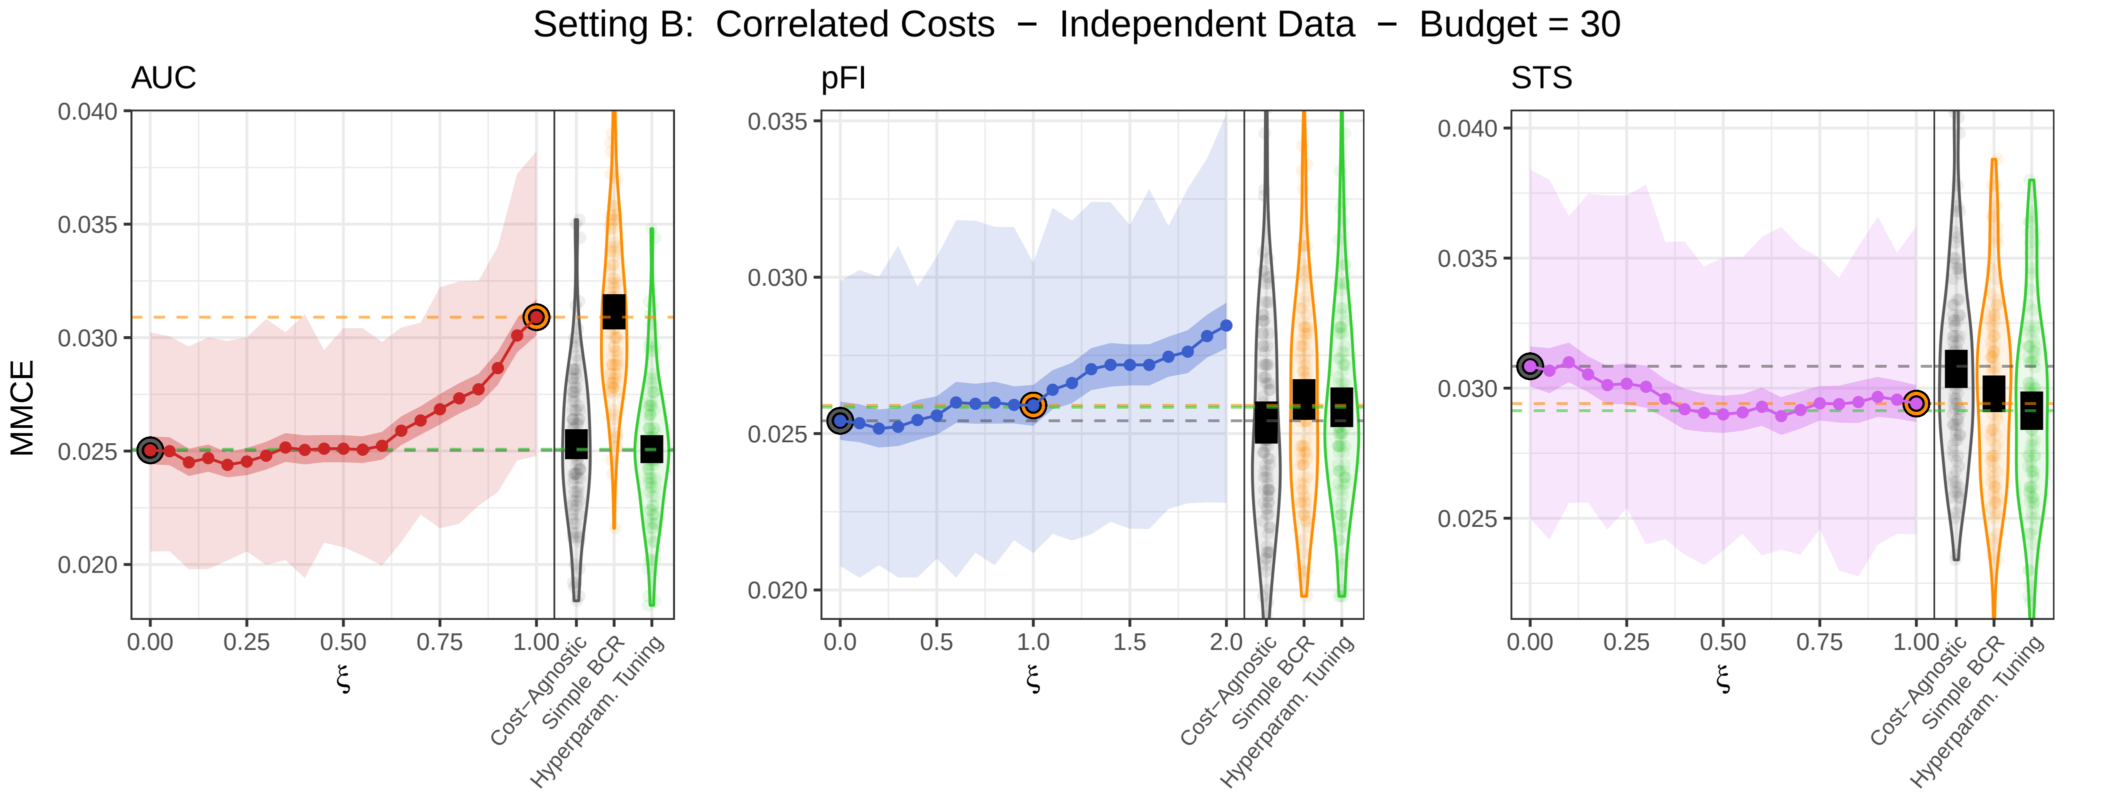
Setting B: Correlated Costs − Independent Data − Budget = 30
AUC
pFI
STS
MMCE
0.040
0.035
0.030
0.025
0.020
0.00
0.25
0.50
0.75
1.00
0.0
0.5
1.0
1.5
2.0
ξ
Cost−Agnostic
Simple BCR
Hyperparam. Tuning

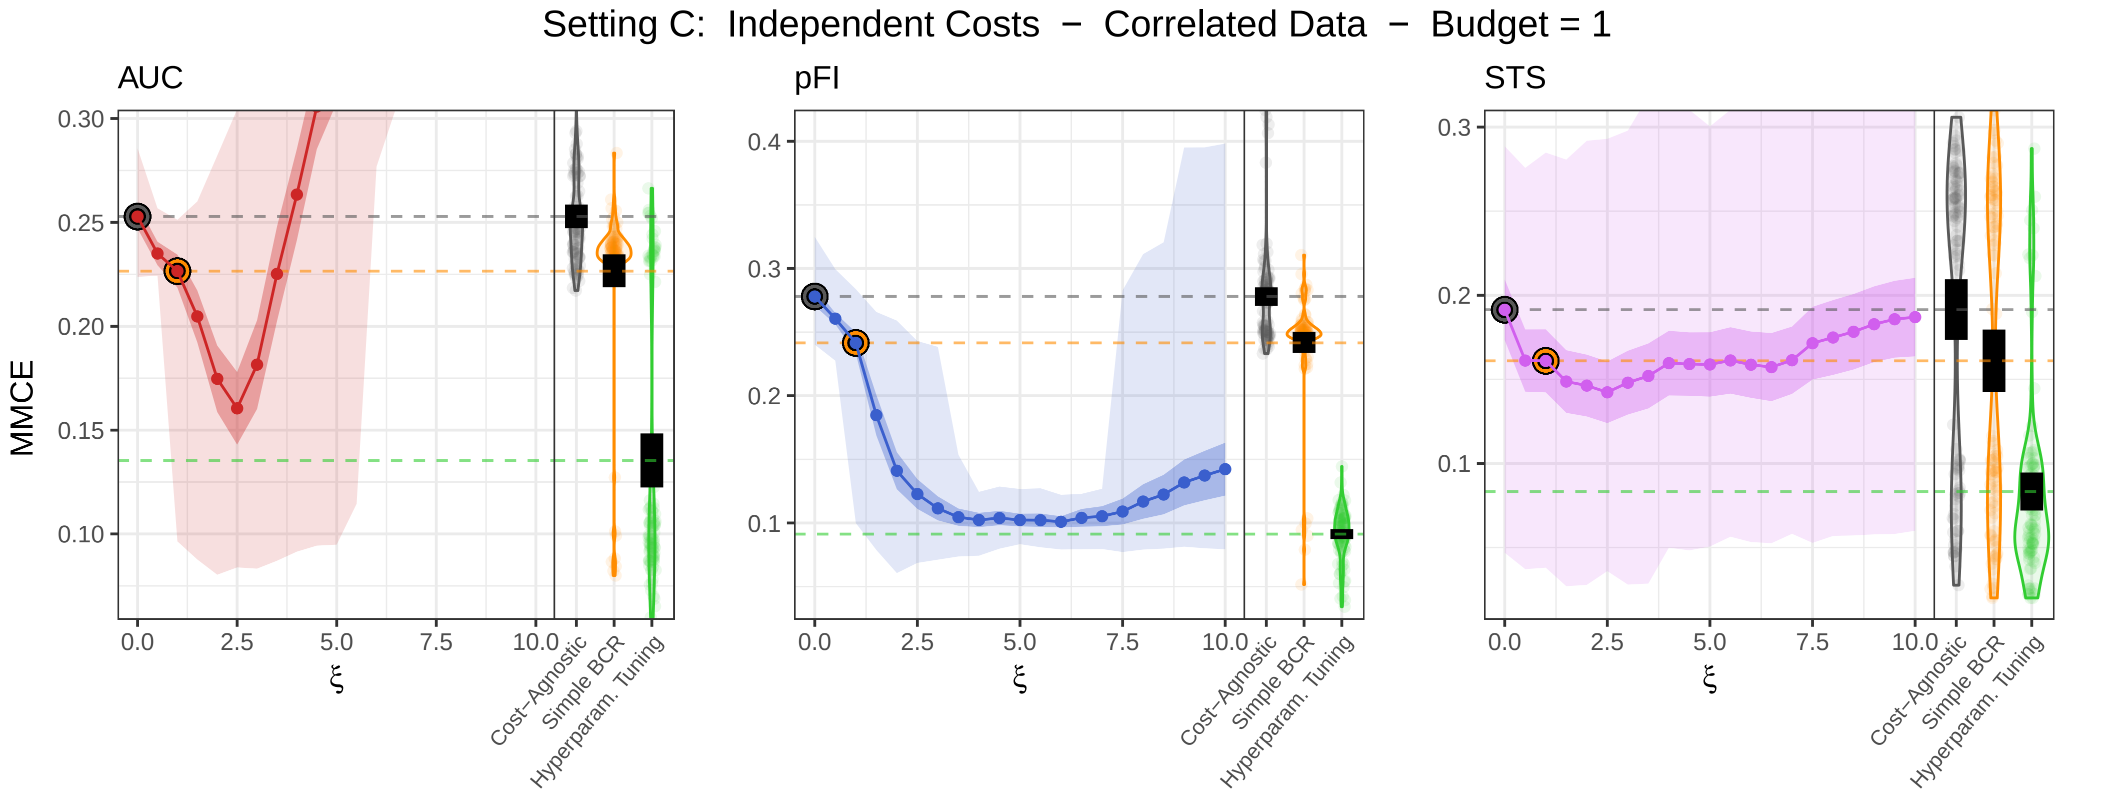
Setting C: Independent Costs − Correlated Data − Budget = 1
AUC
pFI
STS
MMCE
ξ
0.0
2.5
5.0
7.5
10.0
Cost−Agnostic
Simple BCR
Hyperparam. Tuning
0.30
0.25
0.20
0.15
0.10
0.4
0.3
0.2
0.1

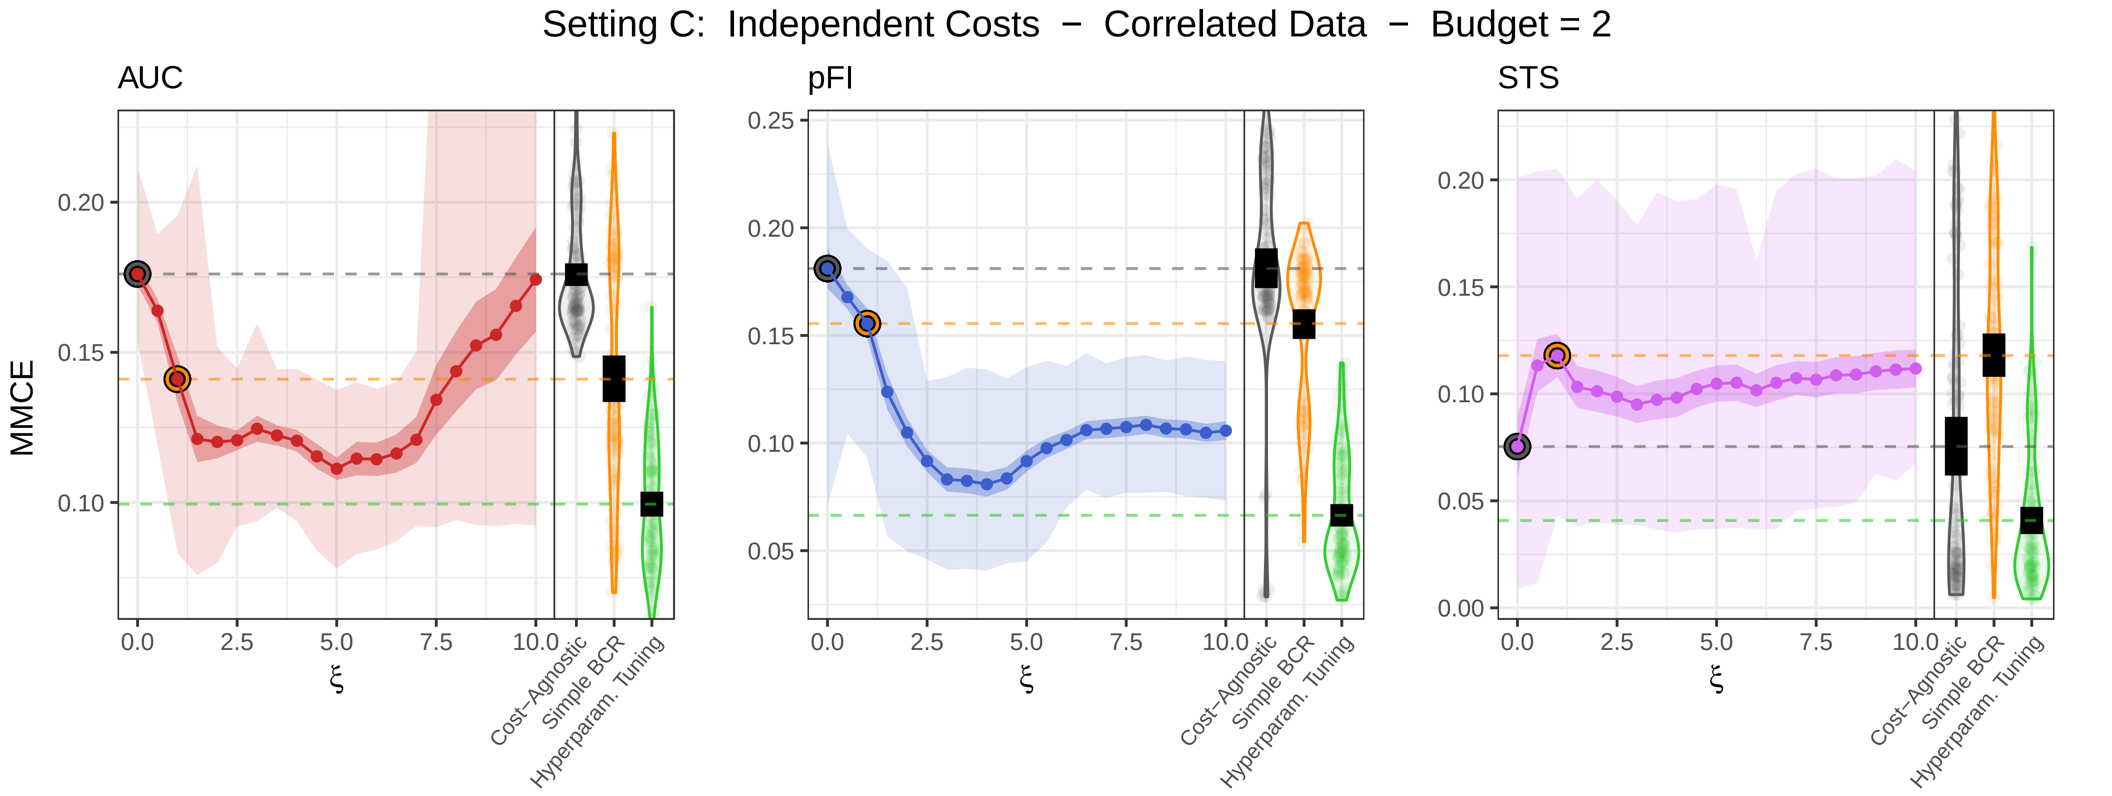

Setting C: Independent Costs − Correlated Data − Budget = 2
AUC
pFI
STS
MMCE
ξ
0.0
2.5
5.0
7.5
10.0
0.10
0.15
0.20
0.05
0.25
0.00
Cost−Agnostic
Simple BCR
Hyperparam. Tuning

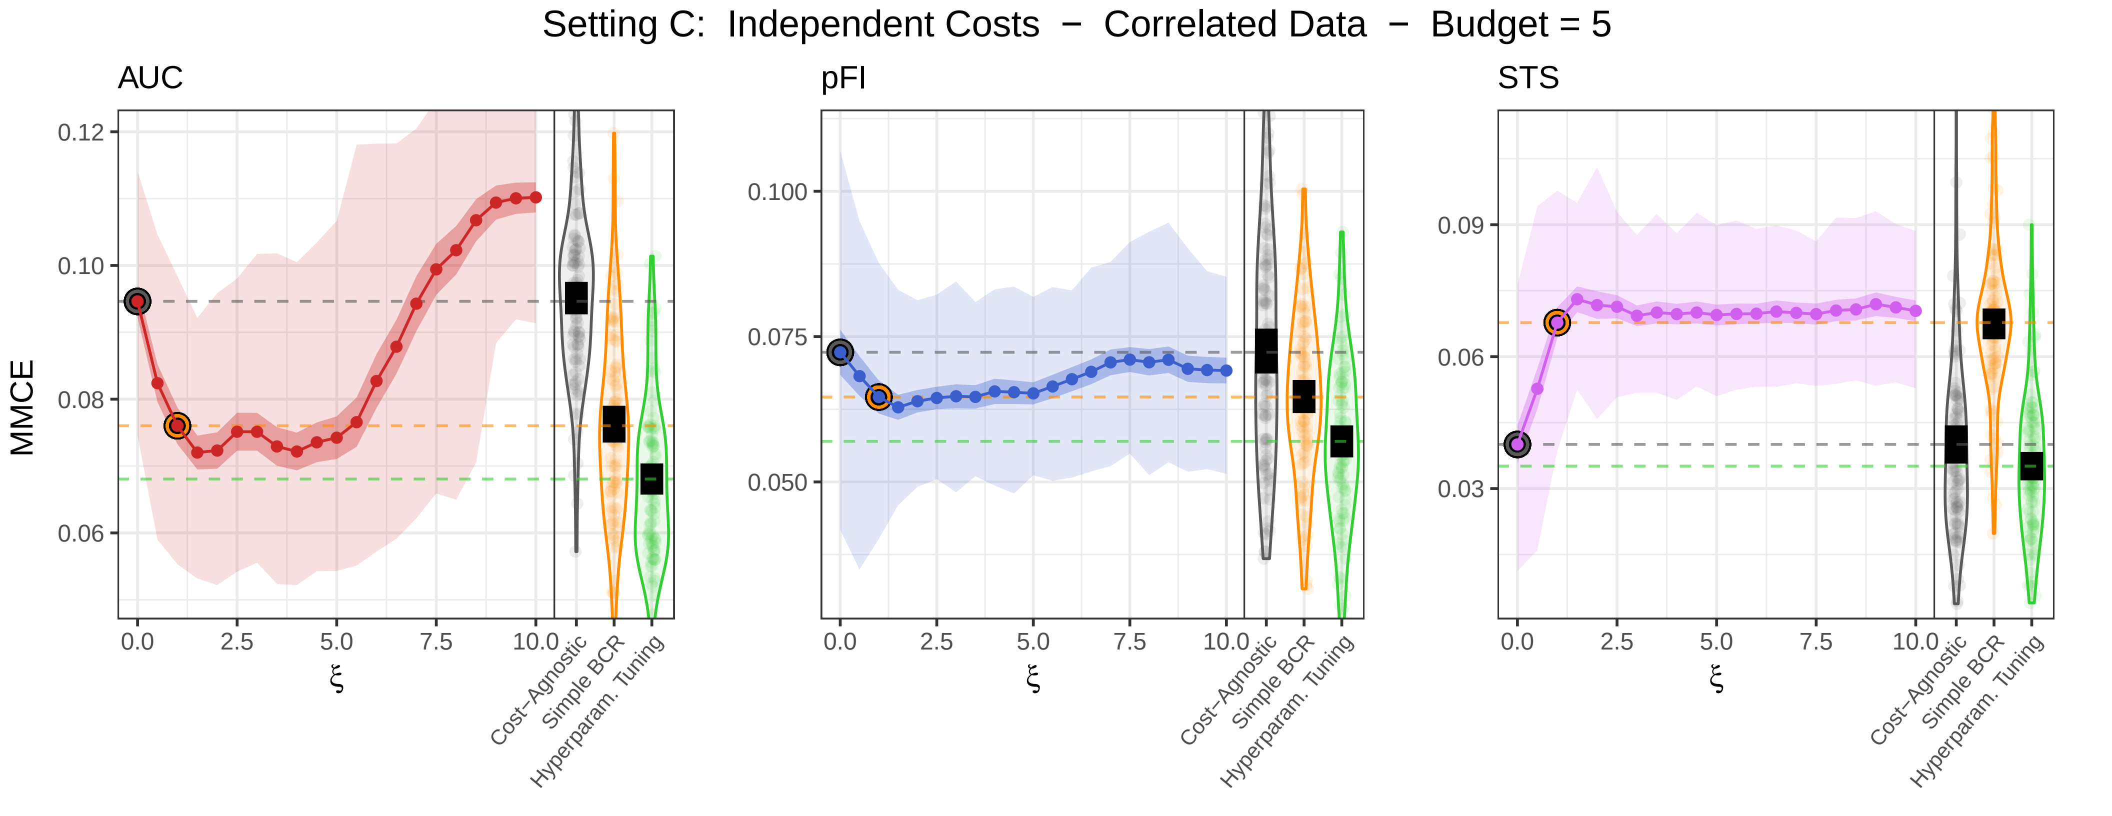

Setting C: Independent Costs − Correlated Data − Budget = 5
AUC
pFI
STS
MMCE
ξ
0.0
2.5
5.0
7.5
10.0
0.06
0.08
0.10
0.12
0.050
0.075
0.100
0.03
0.06
0.09
Cost−Agnostic
Simple BCR
Hyperparam. Tuning

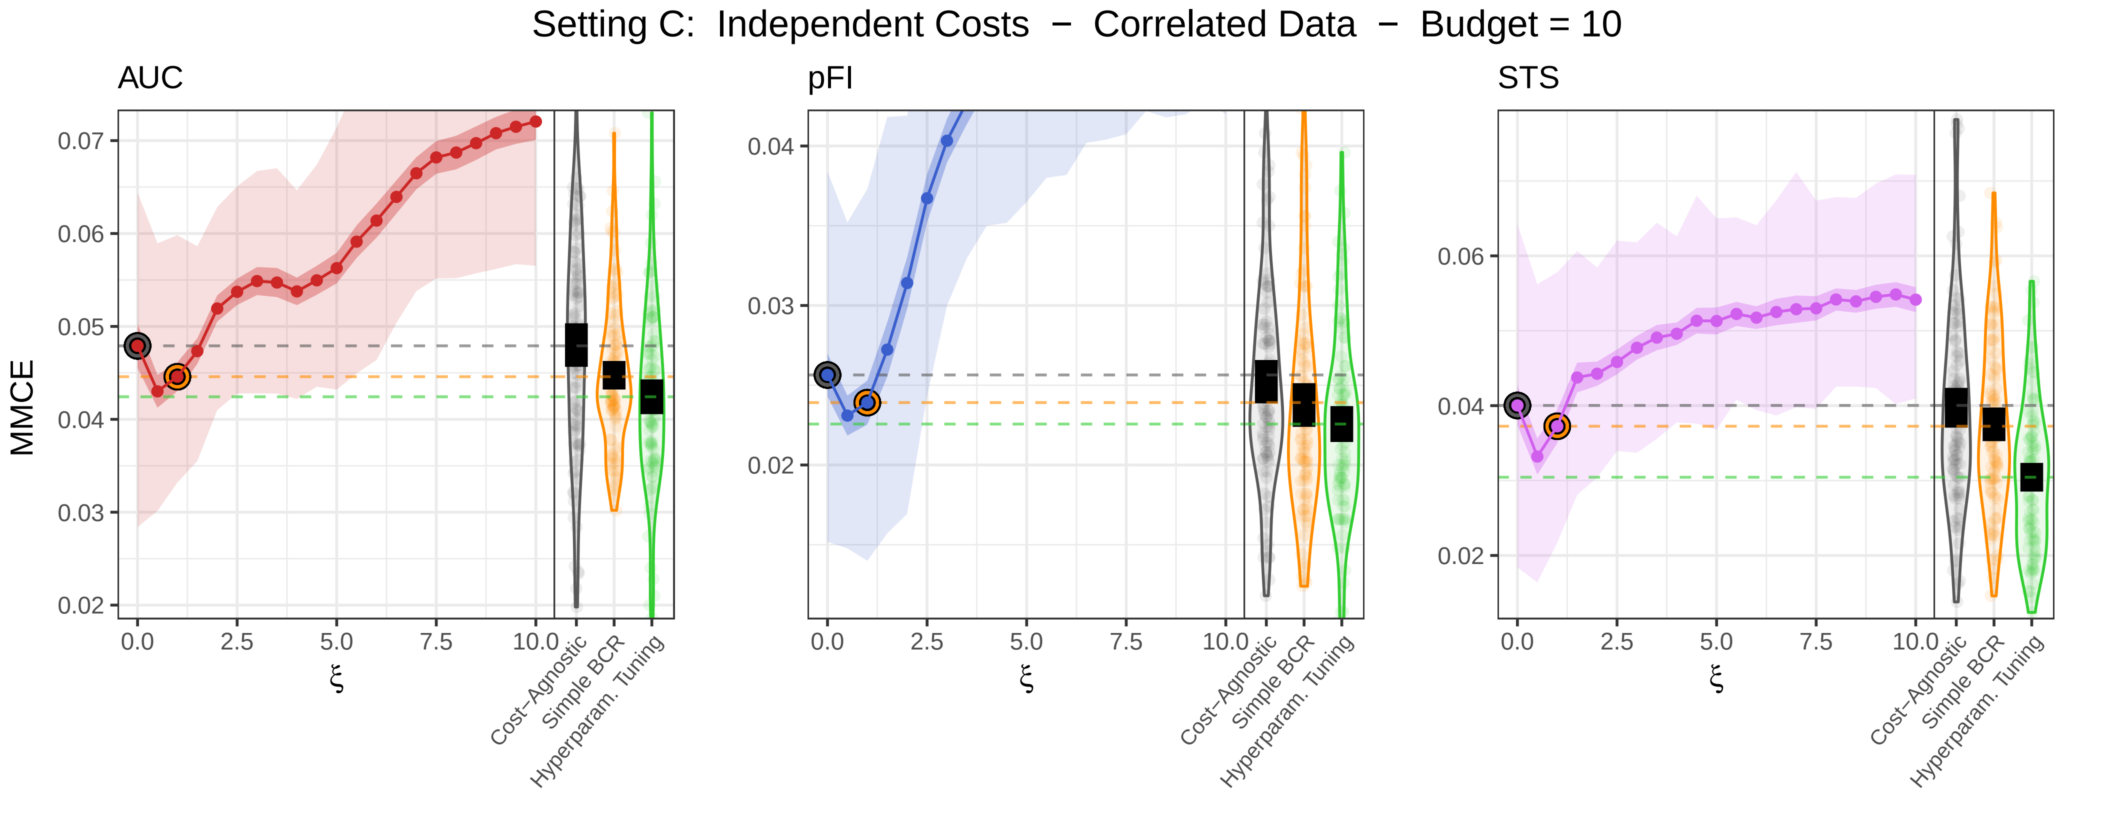

Setting C: Independent Costs − Correlated Data − Budget = 10
AUC
pFI
STS
MMCE
ξ
0.0
2.5
5.0
7.5
10.0
Cost−Agnostic
Simple BCR
Hyperparam. Tuning
0.02
0.03
0.04
0.05
0.06
0.07

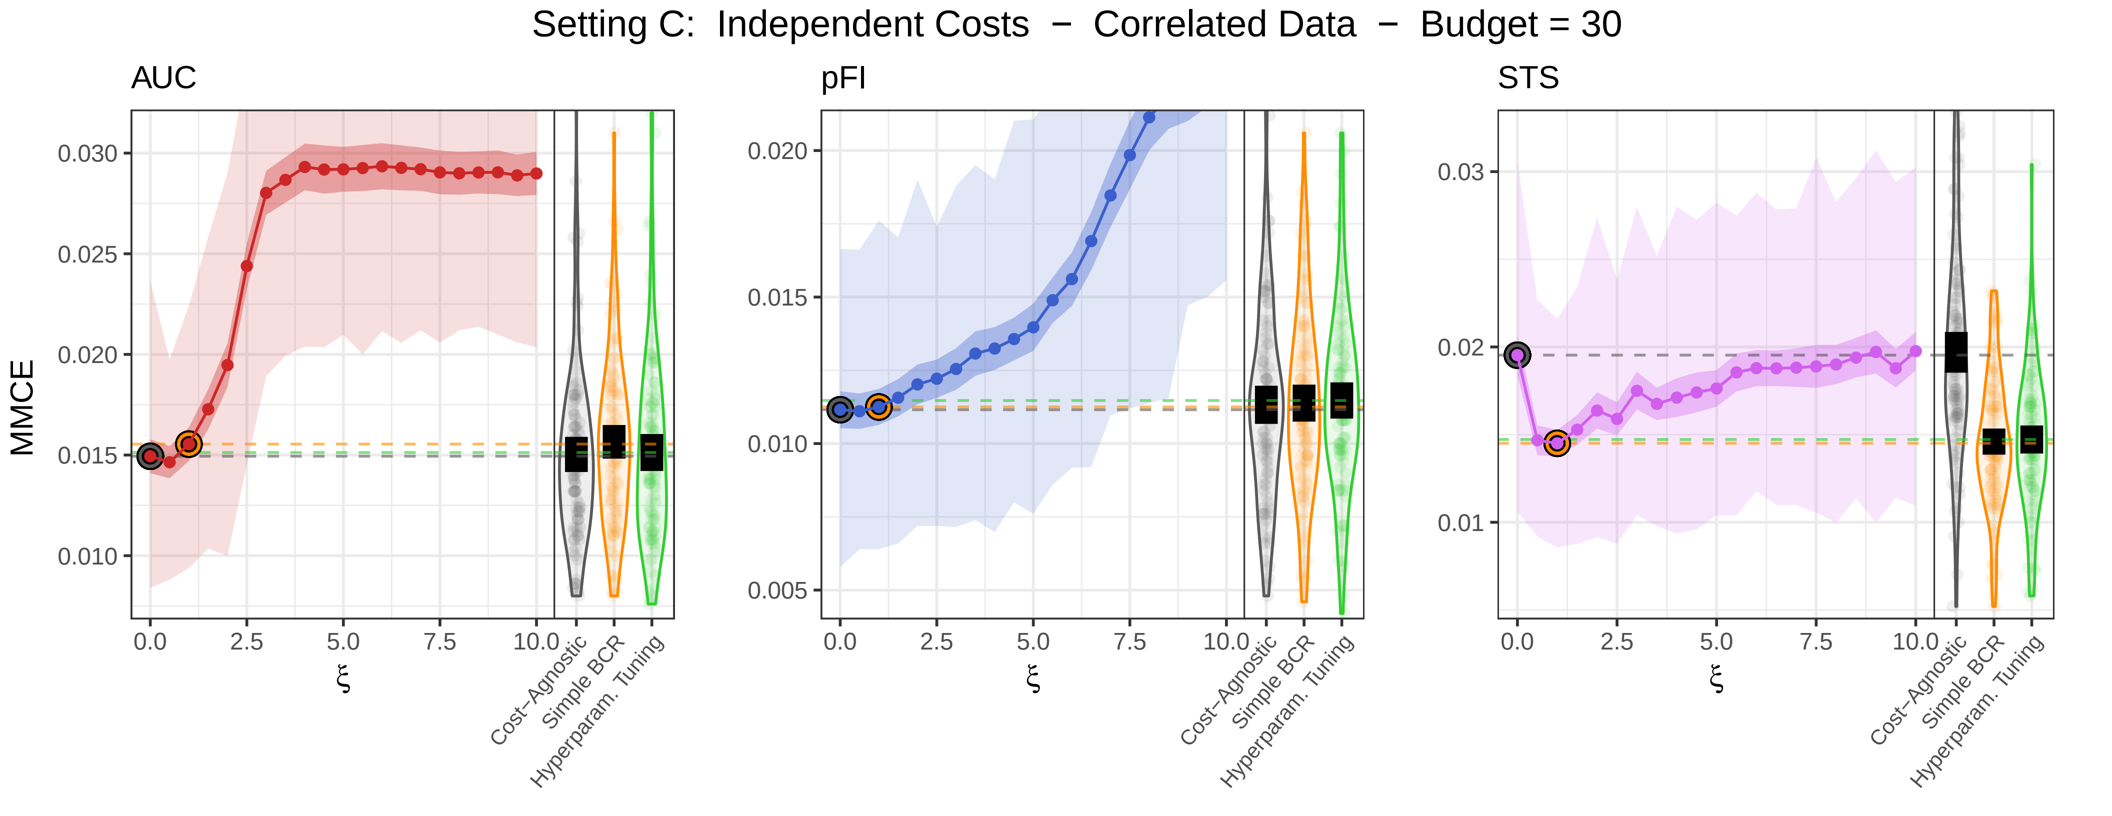

Setting C: Independent Costs − Correlated Data − Budget = 30
AUC
pFI
STS
MMCE
0.030
0.025
0.020
0.015
0.010
0.005
0.03
0.02
0.01
0.0
2.5
5.0
7.5
10.0
ξ
Cost−Agnostic
Simple BCR
Hyperparam. Tuning

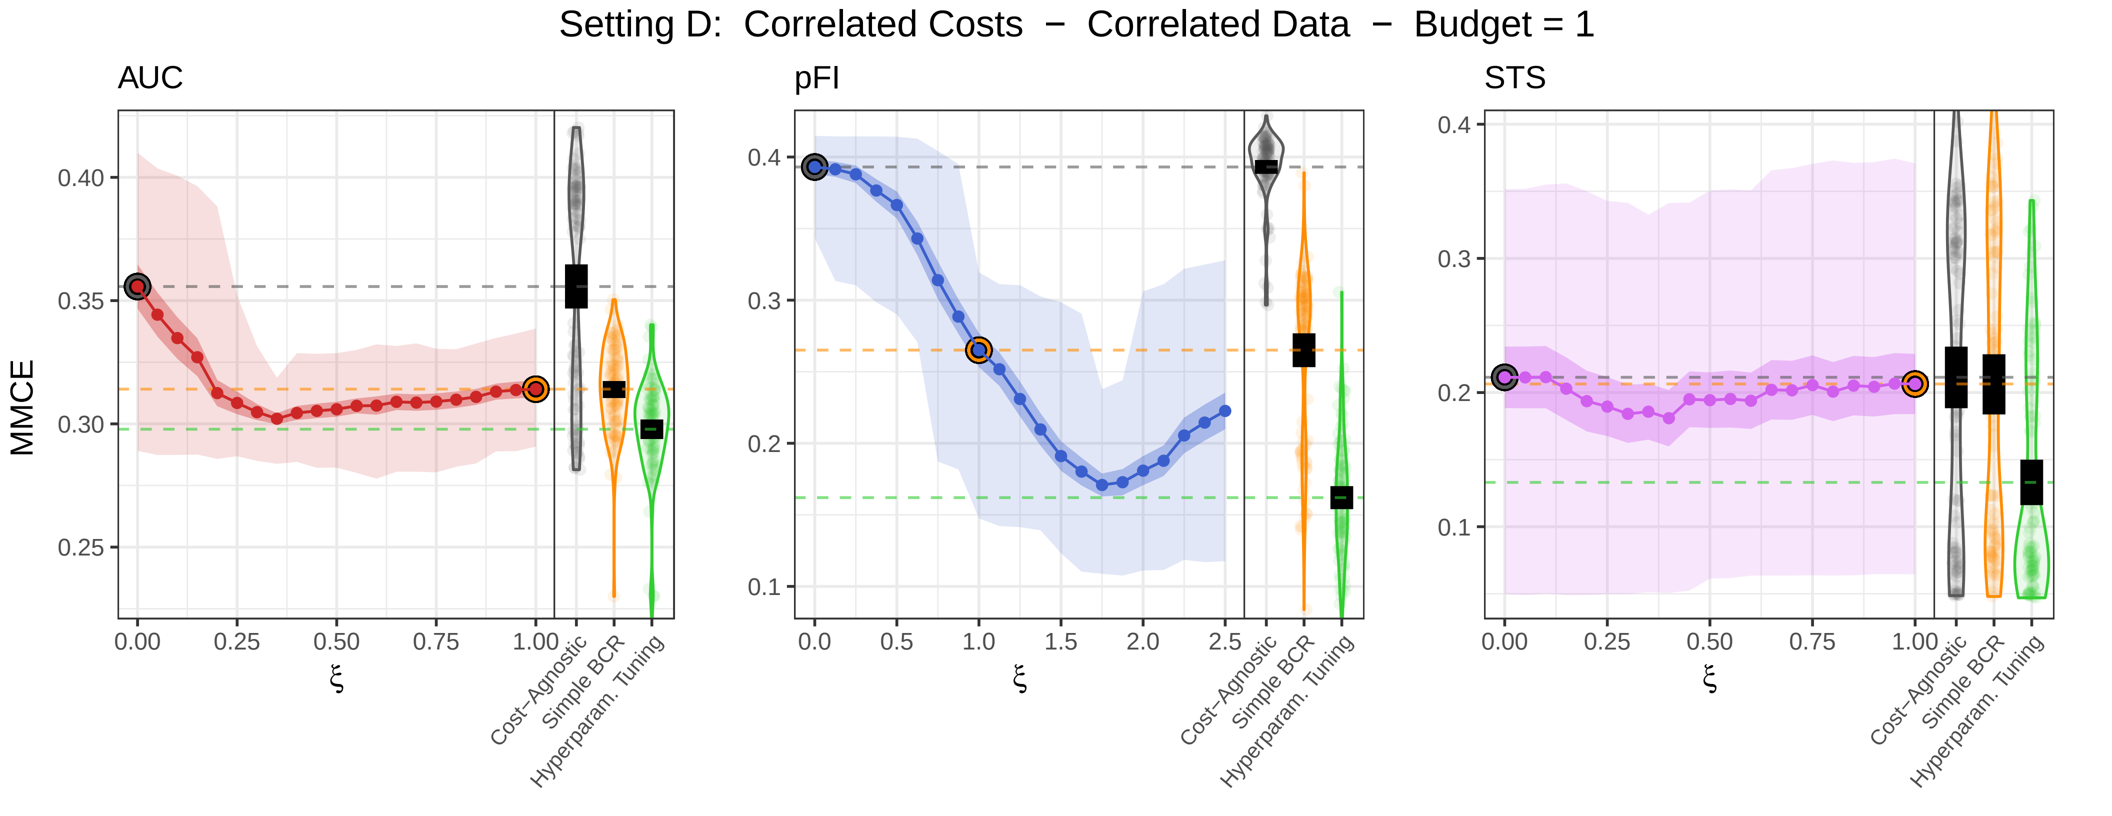
Setting D: Correlated Costs − Correlated Data − Budget = 1
AUC
pFI
STS
MMCE
ξ
0.00
0.25
0.50
0.75
1.00
0.0
0.5
1.0
1.5
2.0
2.5
0.25
0.30
0.35
0.40
0.1
0.2
0.3
0.4
Cost−Agnostic
Simple BCR
Hyperparam. Tuning

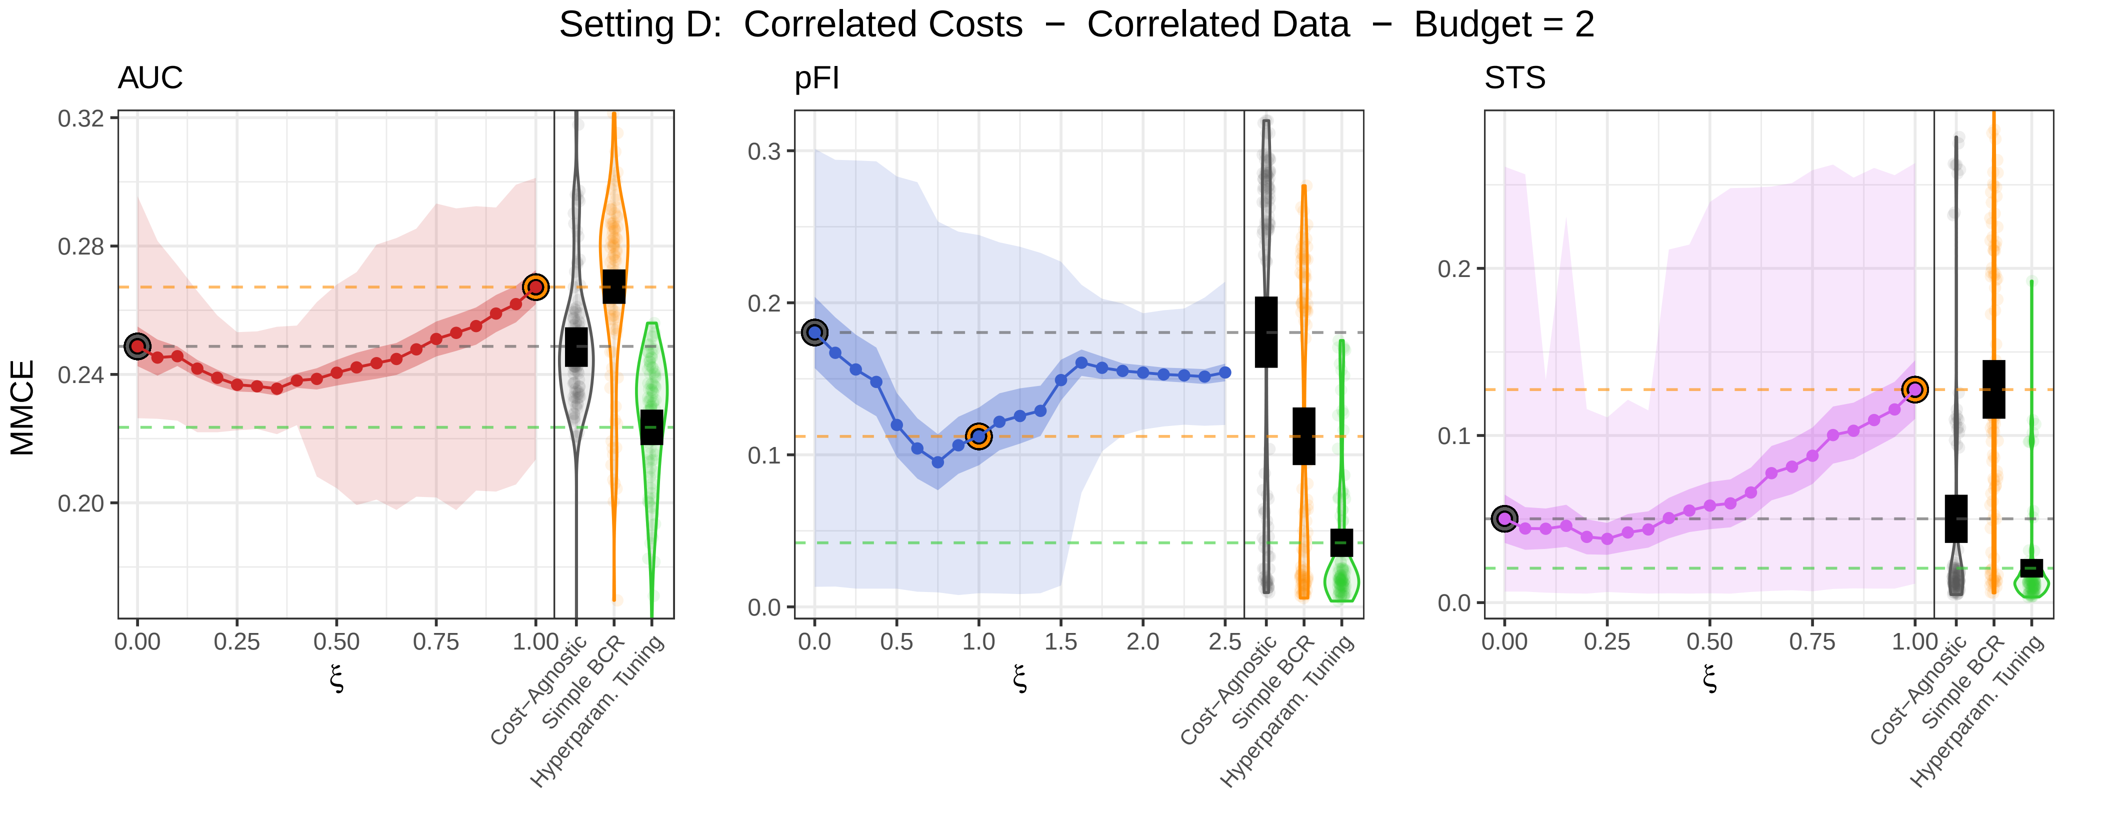
Setting D: Correlated Costs − Correlated Data − Budget = 2
AUC
pFI
STS
MMCE
ξ
Cost−Agnostic
Simple BCR
Hyperparam. Tuning
0.32
0.28
0.24
0.20
0.00
0.25
0.50
0.75
1.00
0.3
0.2
0.1
0.0
0.5
1.0
1.5
2.0
2.5

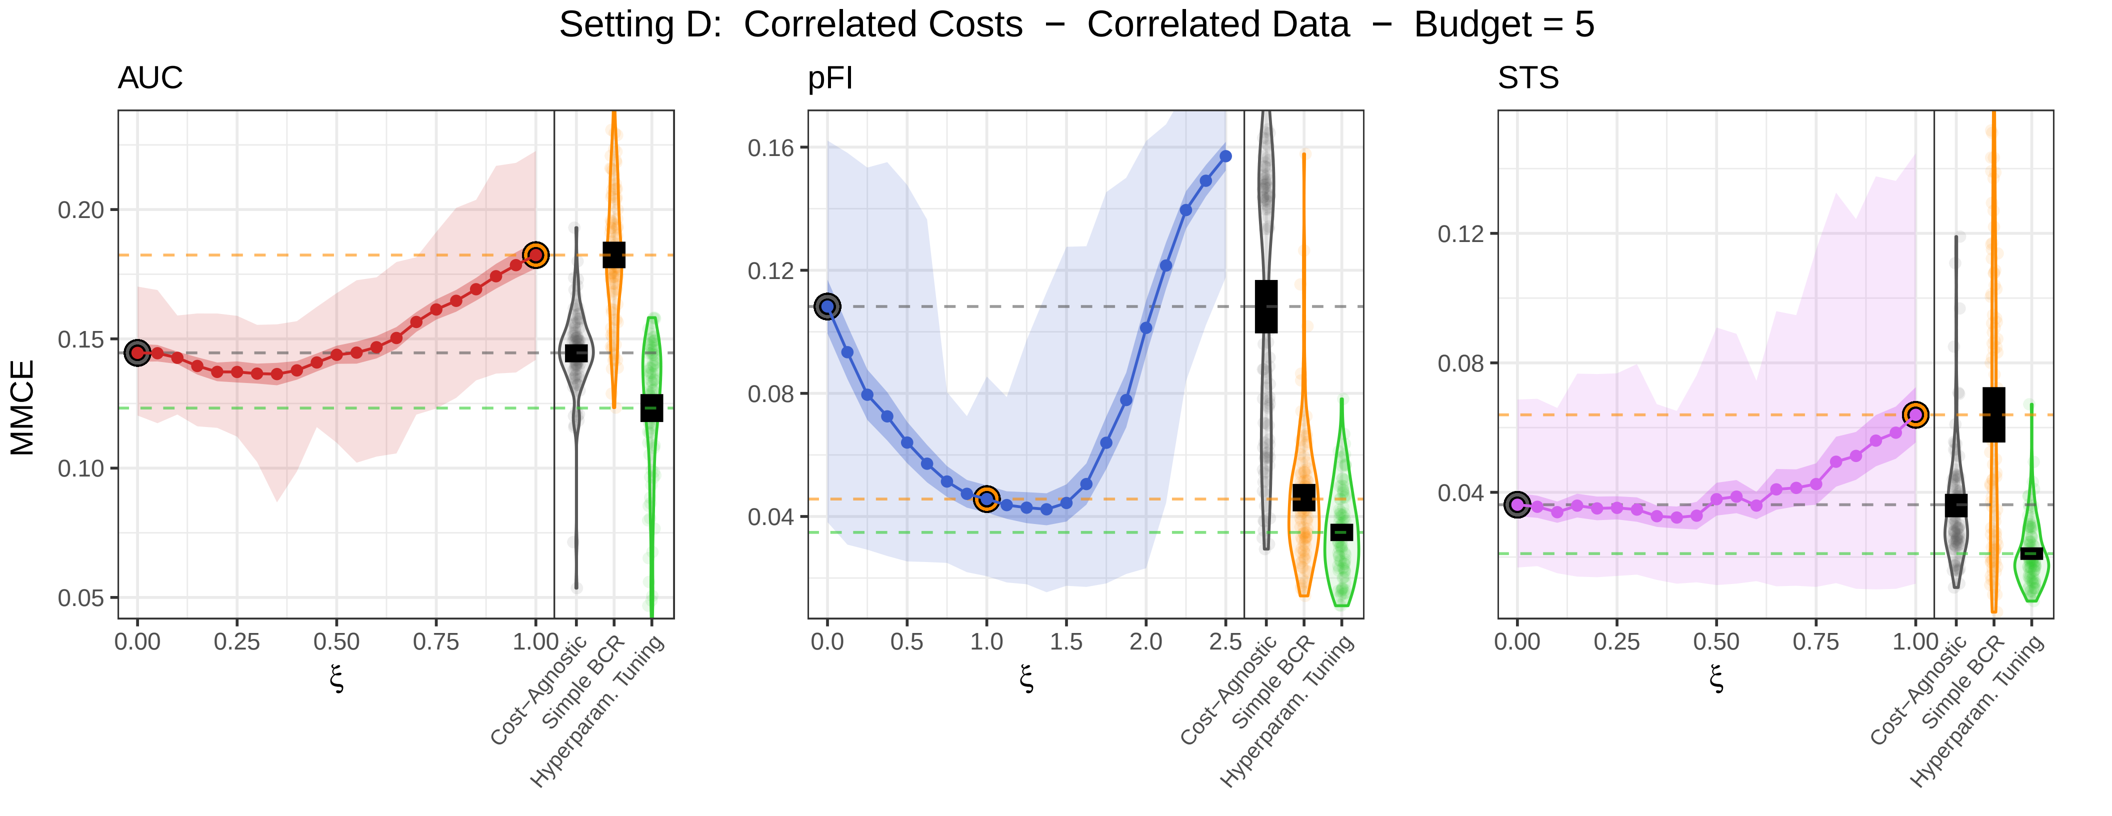
Setting D: Correlated Costs − Correlated Data − Budget = 5
AUC
pFI
STS
MMCE
0.20
0.15
0.10
0.05
0.16
0.12
0.08
0.04
0.12
0.08
0.04
0.00
0.25
0.50
0.75
1.00
0.0
0.5
1.0
1.5
2.0
2.5
ξ
Cost−Agnostic
Simple BCR
Hyperparam. Tuning

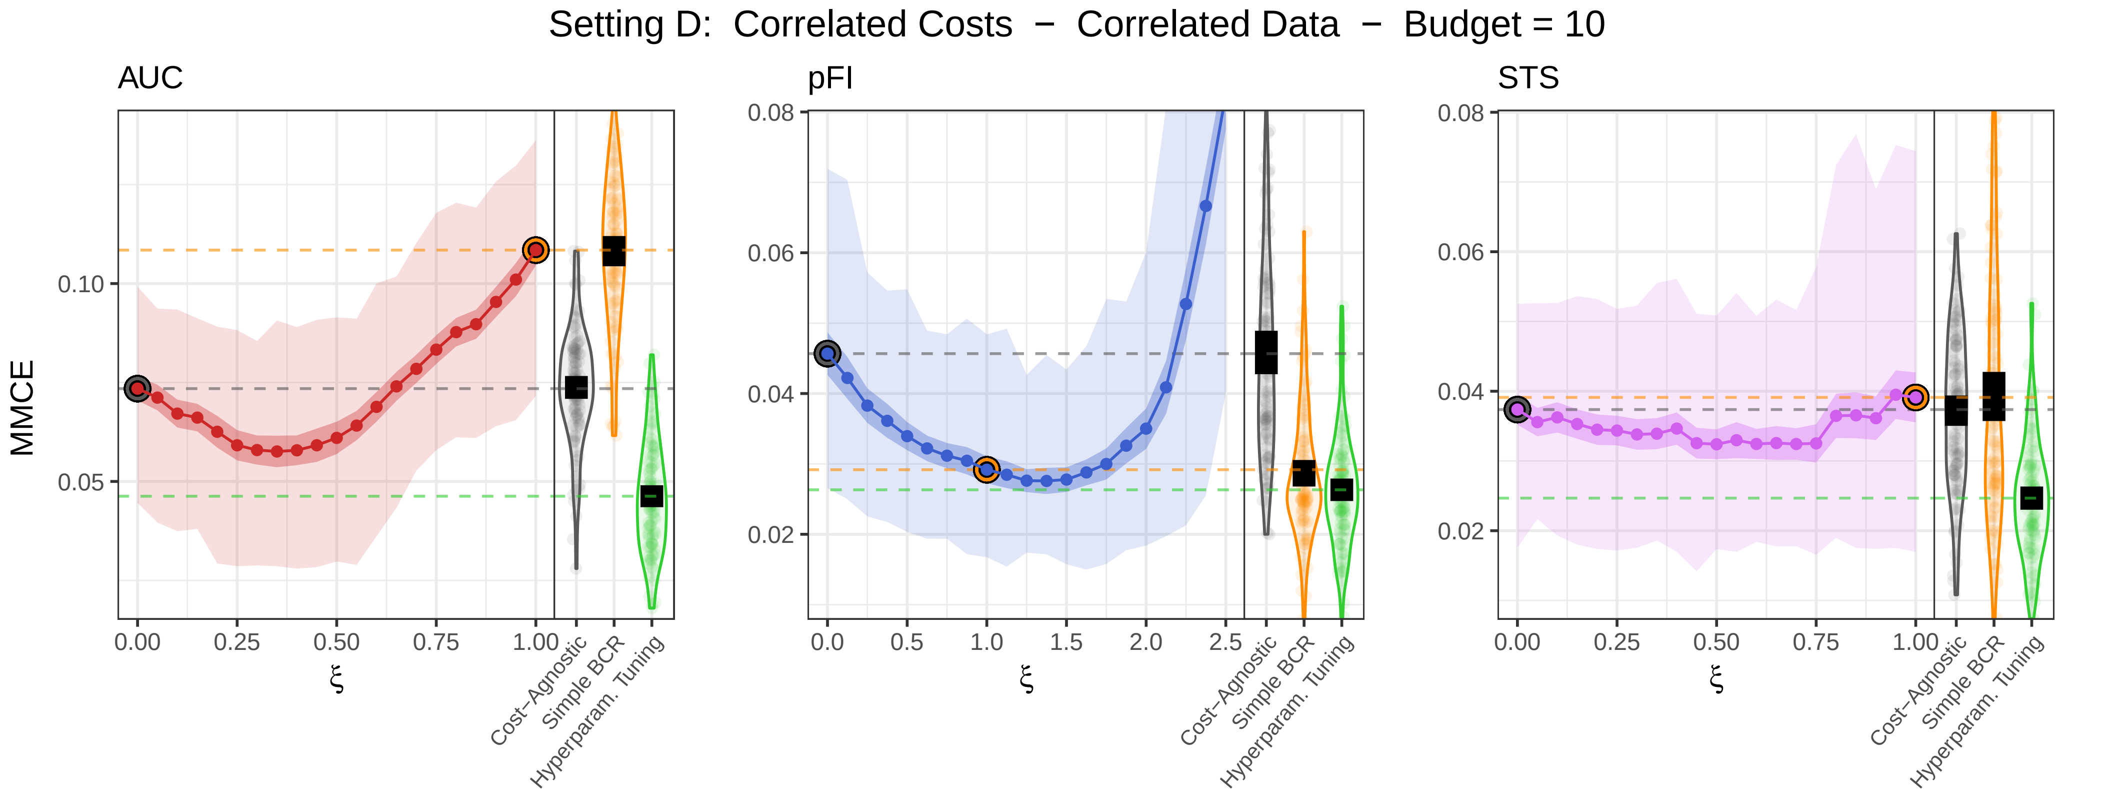

Setting D: Correlated Costs − Correlated Data − Budget = 10
AUC
pFI
STS
MMCE
0.10
0.05
0.08
0.06
0.04
0.02
0.00
0.25
0.50
0.75
1.00
0.0
0.5
1.0
1.5
2.0
2.5
ξ
Cost−Agnostic
Simple BCR
Hyperparam. Tuning

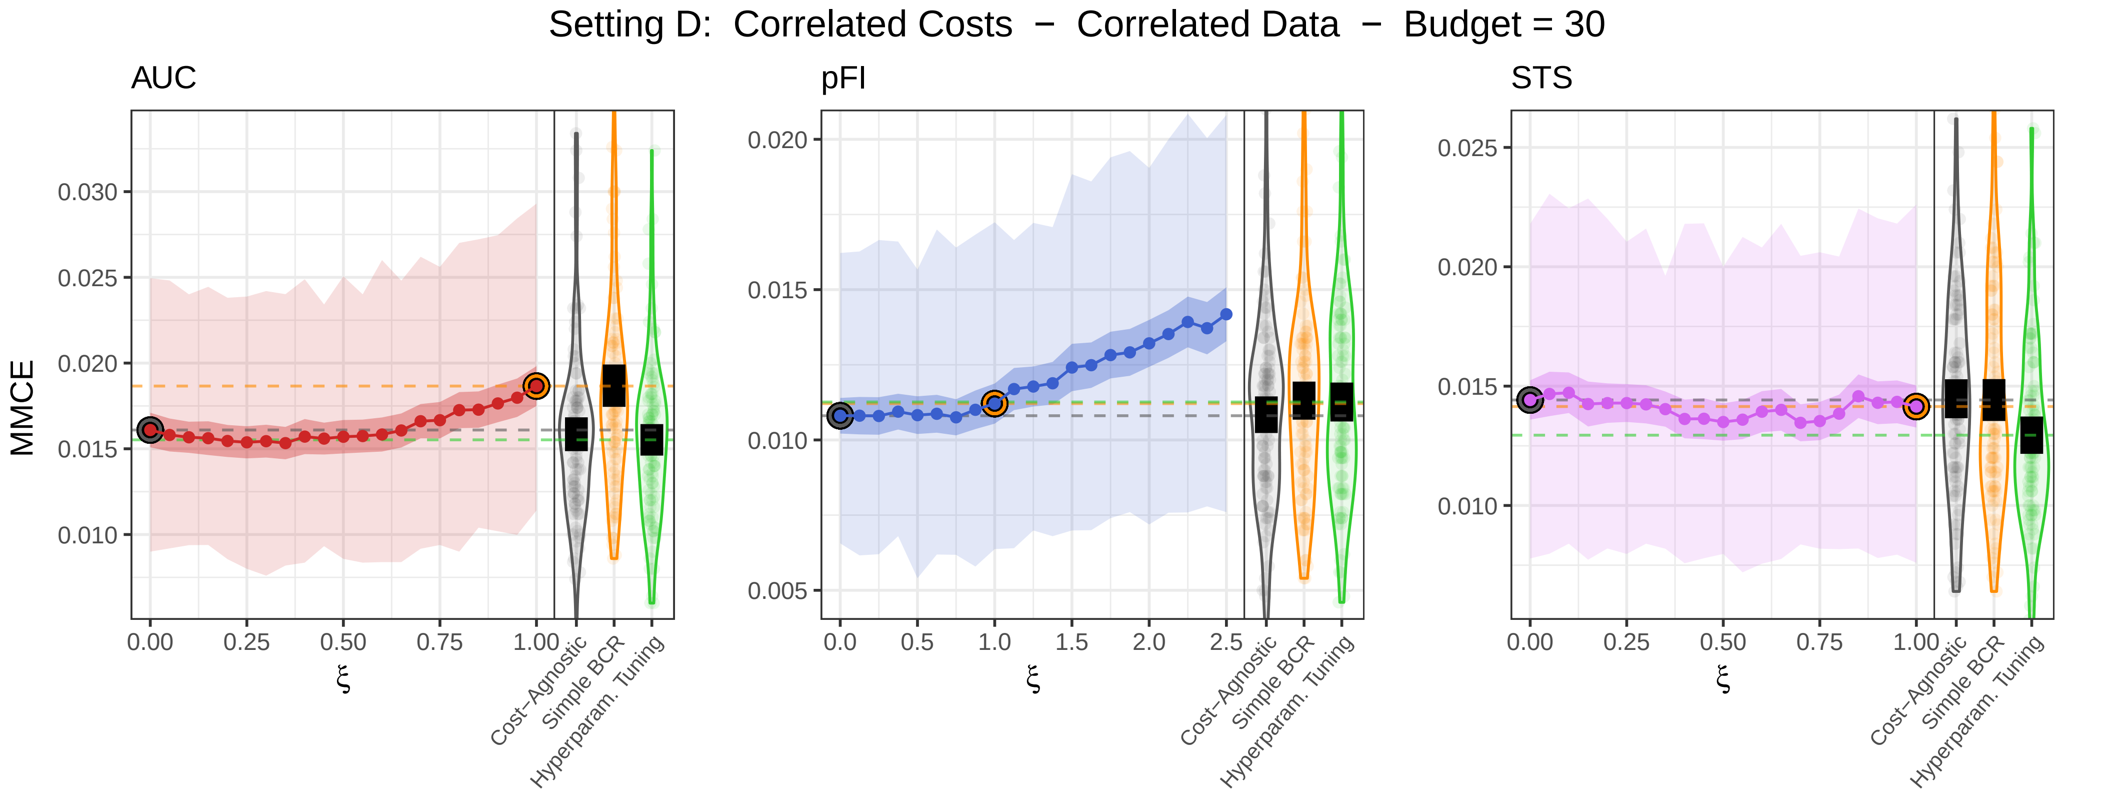

Setting D: Correlated Costs − Correlated Data − Budget = 30
AUC
pFI
STS
MMCE
0.030
0.025
0.020
0.015
0.010
0.00
0.25
0.50
0.75
1.00
ξ
Cost−Agnostic
Simple BCR
Hyperparam. Tuning
0.020
0.015
0.010
0.005
0.0
0.5
1.0
1.5
2.0
2.5
0.025
